# Supplementary material for: Scaling Law for Stochastic Gradient Descent in Quadratically Parameterized Linear Regression
Source: arXiv:2502.09106 source file (2025-02-13)
Supplement: Supplementary file 1 [file Appendix.tex]

\textbf{Additional Notation: }
Bold lowercase letters, for example, $\bold{x} \in \mathbb{R}^d$, denote vectors, while bold uppercase letters, for example, $\mathbf{A} \in \mathbb{R}^{m \times n}$, denote matrices. We apply scalar operators to vectors with the interpretation that these operations should be applied to each coordinate of the vector. For vector $\mathbf{x}\in \mathbb{R}^d$, denote  $\mathbf{\left | x  \right | } \in \mathbb{R}^d$ with $\mathbf{\left | x  \right | }_j = \left | \mathbf{x} _j \right | $. For two vectors $\mathbf{x}, \mathbf{y}\in \mathbb{R}^d$, denote $\mathbf{x}\le \mathbf{y}$, if for all $j\in \left [ d \right ]$, $\mathbf{x}_j\le \mathbf{y}_j$. 

For $\mathbf{v},\mathbf{b}\in\mathbb{R}^M$ with $M \in \mathbb{N}_+$, define $|\mathbf{v}| = (|\mathbf{v}_1|, \ldots, |\mathbf{v}_M|)^{\top}$. Under Assumption \ref{ass-d}, the random variable $\Pi_M \upx \in \mathbb{R}^M$ satisfies the sub-Gaussian condition with parameter $\lambda_i^{1/2}$ for all $i \in [1:M]$, and $\xi$ is sub-Gaussian with parameter $\sigma_{\xi}$.  For any $N\in\bbN_+$, we define
\begin{align}
    &\sigmin(N):=\min_{j\in[1:N]}\lambda_{j}(\upv_j^*)^2,\quad \Barsigmin(N):=\min_{j\in[1:N]}(\upv_j^*)^2,\notag
    \\
    &\Hatsigmax(N):=\max_{j\in[1:N]}\log^{-1}(\upv_j^0),\quad \Tildesigmax(N):=\max_{j\in[N+1:M]}\lambda_j.\notag
\end{align}
We denote the matrix $\diag\{\lambda_1, \dots, \lambda_M\}$ as $\Lambda_{1:M}$. For $\mathbf{b} \in \mathbb{R}_+^M$, define $\mathcal{M}(\mathbf{b}) = (\sum_{j=1}^M \lambda_j \mathbf{b}_j^4)^{1/2}$ and $\sigma^2 = \sigma_{\xi}^2 + \sigma_{\zeta_{M+1:\infty}}^2$, where $\sigma_{\zeta_{M+1:\infty}} = (\sum_{j=M+1}^\infty \lambda_j (\upv_j^*)^4)^{1/2}$.
Given a positive integer $N \leq M$ and a vector $\upv \in \mathbb{R}^M$, denote $\upv_{1:N}$ as $(\upv_1, \ldots, \upv_N)^{\top}$. For a sequence of real numbers $\{v^t\}_{t=t_1}^{t_2}$ and $a, b \in \mathbb{R}$ with $a \leq b$, denote $v^{t_1:t_2} \in [a, b]$ to indicate that $v^t \in [a, b]$ for all $t \in [t_1, t_2]$. Let $\calF^t=\sigma\{\mathbf{v}^0,(\Pi_M\upx^1,\zeta_{M+1:\infty}^1,\xi^1),\cdots,$ $(\Pi_M\upx^t,\zeta_{M+1:\infty}^t,\xi^t)\}$ be the filtration involving the full information of all the previous $t$ times iterations with sigma algebra $\sigma\{\cdot\}$. 

%\begin{definition}[$\calN$-truncation]
%	Considering finite set $\calN\subset\bbN$ is the truncate set and $\mathbf{v}\in\bbR^{\bbN}$, we notate $\mathbf{v}_{\calN}$ a $\#(\calN)$-dimensional vector composed with those dimensions in $\calN$ of $\mathbf{v}$.
%\end{definition}
% \iffalse
% \begin{definition}[$\mathbf{b}$-bounded coupling]
% Let $\{\mathbf{v}^t\}_{t=0}^T$ be a trajectory of  $M$-dimensional positive vectors depend on time $t$. For $\mathbf{b}\in\bbR_+^{M}$, we call sequence $\{\bar{\mathbf{v}}^t\}_{t=0}^T$ a $\mathbf{b}$-bounded coupling based on $\{\mathbf{v}^t\}_{t=0}^T$ if $\{\bar{\mathbf{v}}^t\}_{t=0}^T$ starts from $\bar{\mathbf{v}}^0=\mathbf{v}^0$ where $\mathbf{v}^0\leq\mathbf{b}$, for each time $t<T$, if $\bar{\mathbf{v}}^t\leq\mathbf{b}$, we let $\bar{\mathbf{v}}^{t+1}=\mathbf{v}^{t+1}$; otherwise $\bar{\mathbf{v}}^{t+1}=\bar{\mathbf{v}}^t$.
% %$\calB_{\mathbf{b},\gamma}(\mathbf{v}^*)$
% \end{definition}
%\begin{definition}[$(\mathbf{b},\gamma)$-bounded potential function of $\calN$-truncation]
%	For a vector $\mathbf{v}\in\bbR_+^n$ ($n\in\bbN$ can be infinite), $\mathbf{b}\in\bbR_+^{\#(\calN)}$ and $\gamma>0$, we call function $\phi:\bbR_+^n\rightarrow\bbR_+$ a $(\mathbf{b},\gamma)$-bounded potential function of $\calN$-truncation if
%	\begin{align}
%		\phi(\mathbf{v})=\begin{cases}
%			\sum_{i\in\bar{\calN}}\sqrt{\mathbf{v}_i}, & \text{ if }|\mathbf{v}_{\calN}|\leq\mathbf{b}\text{ and }\|\mathbf{v}_{\bar{\calN}}\|_1\leq\gamma,
%			\\
%			0, & \text{ otherwise }.
%		\end{cases}
%	\end{align}
%\end{definition}
\subsection{Preliminary}
Recall that $\upx$ denote the covariate vector in $\bbH$. Let $\{\upu_i\}_{i=1}^{\infty}$ be an orthonormal basis of $\bbH$ and $\upx_i=\langle\upx,\upu_i\rangle$ for any $i\in[1:\infty]$. The projection operator $\Pi_M:\upH\rightarrow\bbR^M$ is defined as $\Pi_M=\sum_{i=1}^M\upe_i\otimes\upu_i$. One can notice the projection $\Pi_M\upx$ satisfies $\Pi_M\upx=(\upx_1,\cdots,\upx_M)^{\top}$. Define the random variable $\zeta_{M+1:\infty}=\sum_{i=M+1}^{\infty}\upx_i(\upv_i^*)^2$. At the $t$-th iteration, Algorithm \ref{SGD} requires sampling $(\Pi_M\upx^t,y^t)$ , which is equivalent with sampling the triplet $(\Pi_M\upx^t,\zeta_{M+1:\infty}^t,\xi^t)$. For each iteration $t$, we define the events, \congfang{which simply rule out some low-probabilistic unbounded cases???}.
\begin{align}
    &\calE_1^{j,t}:=\left\{\left|\upx_j^t\right|\leq\lambda_j^{1/2}R\right\}, \quad \calE_2^{j,t}:=\left\{\left|\langle\upv^{(t-1)\odot2}-\upv_{1:M}^{*\odot2},\Pi_M\upx^{t}\rangle_{-j}\right|\leq r_j(\upv^{t-1})R\right\}, \quad \forall j\in[1:M],\notag
    \\
    &\, \, \, \, \, \, \, \, \, \, \, \, \, \, \, \, \, \, \, \, \, \, \, \, \, \, \, \, \, \, \, \, \, \, \, \, \, \, \, \, \, \, \, \, \, \calE_3^t:=\left\{\left|\zeta_{M+1:\infty}^t\right|\leq\sigma_{\zeta_{M+1:\infty}}R\right\}, \quad \calE_4^t:=\left\{\left|\xi^t\right|\leq\sigma_{\xi}R\right\},\notag
\end{align}
where $R:=\calO(\log(MT/\delta))$ and $r_j(\upw):=\calO(\sum_{i\neq j}\lambda_i[(\upw_i)^4+(\upv_i^*)^4])^{1/2}$ for any $\upw\in\bbR^M$. From Assumption \ref{ass-d} and Proposition \ref{prop-A5}, it follows that
\begin{align}
    \min\left\{\bbP\left(\calE_1^{j,t}\right),\bbP\left(\calE_2^{j,t}\right),\bbP\left(\calE_3^{t}\right),\bbP\left(\calE_4^{t}\right)\right\}\geq 1-\calO\left(\frac{\delta}{MT^2}\right),\quad \forall j\in[1:M] \text{ and } t\in[1:T].\notag
\end{align}
Define the compound event $\calE:=\left\{\bigcap_{t=1}^T\left(\left(\bigcap_{j=1}^M\calE_1^{j,t}\right)\bigwedge\left(\bigcap_{j=1}^M\calE_2^{j,t}\right)\bigwedge\calE_3^t\bigwedge\calE_4^t\right)\right\}$. Then, we applying the probability union bound as follows:
\begin{align}
    \bbP(\calE)=1-\bbP(\calE^c)\geq&1-\sum_{t=1}^T\left(2-\bbP(\calE_3^t)-\bbP(\calE_4^t)+\sum_{j=1}^M\left(2-\bbP\left(\calE_1^{j,t}\right)-\bbP\left(\calE_2^{j,t}\right)\right)\right)\notag
    \\
    \geq&1-\calO\left(\frac{\delta}{T}\right).
\end{align}

According to Algorithm \ref{SGD}, the original sequence $\{\upv^t\}_{t=0}^T$ follows the coordinate-wise update rule:
\begin{equation}
    \begin{split}
    \upv_j^{t+1}=&\upv_j^t-\eta_t\left(\langle\upv^{t\odot2},\Pi_M\upx^{t+1}\rangle-y^{t+1}\right)\upx_j^{t+1}\upv_j^t\\
    \notag
    =&\upv_j^t-\eta_t\llangle\upv^{t\odot2}-\upv_{1:M}^{*\odot2},\Pi_M\upx^{t+1}\rrangle\upx_j^{t+1}\upv_j^t+\eta_t\left(\zeta_{M+1:\infty}^{t+1}+\xi^{t+1}\right)\upx_j^{t+1}\upv_j^{t},
    \end{split}\notag
\end{equation}
for any $j\in[1:M]$. Leveraging the high-probability property of event $\calE$, we analyze the coordinate-wise update dynamics for the control sequence $\{\upq^t\}_{t=0}^{T}$ in $\bbR^M$:
\begin{align}\label{update-q-primal}
    \upq_j^{t+1}=\upq_j^t&-\eta_t\left(\left(\upq_j^t\right)^2-\left(\upv_j^*\right)^2\right)\left(\upx_j^{t+1}\right)^2\mathds{1}_{|\upx_j^{t+1}|\leq\lambda_j^{1/2}R}\upq_j^t\notag
    \\
    &-\eta_t\llangle\upq^{t\odot2}-\upv_{1:M}^{*\odot2},\Pi_M\upx^{t+1}\rrangle_{-j}\mathds{1}_{|\langle\upq^{t\odot2}-\upv_{1:M}^{*\odot2},\Pi_M\upx^{t+1}\rangle_{-j}|\leq r_j(\upq^t)R}\upx_j^{t+1}\mathds{1}_{|\upx_j^{t+1}|\leq\lambda_j^{1/2}R}\upq_j^t\notag
    \\
    &+\eta_t\left(\zeta_{M+1:\infty}^{t+1}\mathds{1}_{\left|\zeta_{M+1:\infty}^t\right|\leq\sigma_{\zeta_{M+1:\infty}}R}+\xi^{t+1}\mathds{1}_{\left|\xi^t\right|\leq\sigma_{\xi}R}\right)\upx_j^{t+1}\mathds{1}_{|\upx_j^{t+1}|\leq\lambda_j^{1/2}R}\upq_j^t,
\end{align}
for any $j\in[1:M]$ with initialization $\upq^0=\upv^0$. The following probabilistic guarantee holds for all iterations.
\begin{proposition}\label{p1}
    For any $t\in[1:T]$, we have $\upv^{t}=\upq^{t}$ with probability at least $1-\delta/T$.
\end{proposition}
To simplify notations, we introduce four truncated random variables:
\begin{enumerate}
    \item $\widehat{\upx}\in\bbR^M$ with entries $\widehat{\upx}_j=\upx_j\mathds{1}_{|\upx_j|\leq\lambda_j^{1/2}R}$ for any $j\in[1:M]$,
    \item $\widehat{\upz}(\upq)\in\bbR^M$ with entries $\widehat{\upz}_j(\upq)=\llangle\upq^{\odot2}-\upv_{1:M}^{*\odot2},\Pi_M\upx\rrangle_{-j}\mathds{1}_{|\langle\upq^{\odot2}-\upv_{1:M}^{*\odot2},\Pi_M\upx\rangle_{-j}|\leq r_j(\upq)R}$
    \item $\widehat{\zeta}_{M+1:\infty}=\zeta_{M+1:\infty}\mathds{1}_{\zeta_{M+1:\infty}\leq \sigma_{\zeta_{M+1:\infty}}R}$,
    \item $\widehat{\xi}=\xi\mathds{1}_{\xi\leq \sigma_{\xi}R}$. 
\end{enumerate}
Then, the coordinate-wise update dynamics for $\{\upq^{t}\}_{t=0}^T$ in Eq.~\eqref{update-q-primal} reduces to:
\begin{align}\label{update-q}
    \upq_j^{t+1}=\upq_j^t-\eta_t\left(\left(\upq_j^t\right)^2-\left(\upv_j^*\right)^2\right)\left(\widehat{\upx}_j^{t+1}\right)^2\upq_j^t-\eta_t\widehat{\upz}_j^{t+1}(\upq^t)\widehat{\upx}_j^{t+1}\upq_j^t+\eta_t\left(\widehat{\zeta}_{M+1:\infty}^{t+1}+\widehat{\xi}^{t+1}\right)\widehat{\upx}_j^{t+1}\upq_j^t,
\end{align}
for any $j\in[1:M]$. \congfang{???eq}
% The control sequence $\{\upq^t\}_{t=0}^{T}$ follows the coordinate-wise update rule:
% \begin{align}
%      \upq_j^{t+1}=\upq_j^t-\eta_t\llangle\upq^{t\odot2}-\upq_{1:M}^{*\odot2},\widehat{\upx}_{1:M}^{t+1}\rrangle\widehat{\upx}_j^{t+1}\upq_j^t+\eta_t\left(\widehat{\zeta}_{M+1:\infty}^{t+1}+\widehat{\xi}^{t+1}\right)\widehat{\upx}_j^{t+1}\upq_j^{t},\quad \forall j\in[1:M],\notag
% \end{align}
% with initialization $\upq^0=\upv^0$. When $\mathcal{E}$ holds, the trajectories $\{\upv^t\}_{t=1}^{T}$ and $\{\upq^t\}_{t=1}^T$ coincide, yielding $\upv^{t'}=\upq^{t'}$ for any fixed $t'\in[1:T]$ with probability at least $1-\delta$. Therefore, throughout Phase I and the initial segment of Phase II, our analysis focuses on deriving high-probability bounds through the dynamics of $\upq^t$.

\begin{definition}[$\mathbf{b}$-capped coupling]
  Let $\{\mathbf{q}^t\}_{t=0}^T$ be a Markov chain in $\mathbb{R}_+^M$ adapted to filtration $\{\mathcal{F} ^{t}\}_{t=0}^T$. Given threshold vector $\mathbf{b}\in\bbR_+^{M}$, the $\mathbf{b}$-capped coupling process $\{\bar{\mathbf{v}}^t\}_{t=0}^T$ with initialization $\bar{\mathbf{v}}^0=\mathbf{q}^0\le \mathbf{b}$ evolves as:
  \begin{enumerate}
      \item Updating state: If $\bar{\mathbf{v}}^t\le \mathbf{b}$, let $\bar{\mathbf{v}}^{t+1}=\mathbf{q}^{t+1}$,
      \item Absorbing state: Otherwise, maintain $\bar{\mathbf{v}}^{t+1}=\bar{\mathbf{v}}^{t}$. 
  \end{enumerate} 
\end{definition}

\begin{definition}[$(c\mathbf{v}^*_{1:N},\mathbf{b})$-neighbor coupling]
Let $\{\mathbf{q}^t\}_{t=0}^T$ be a Markov chain in $\mathbb{R}_+^M$ adapted to filtration $\{\mathcal{F} ^{t}\}_{t=0}^T$.  Given parameters: 1) Dimension index $N\in \mathbb{Z}_{+}$; 2) Tolerance $c>0$; 3) Threshold vector $\mathbf{b}\in\bbR_+^{M-N}$. With initial condition $\bar{\mathbf{v}}^0=\upq^0$, $\left | \bar{\mathbf{v}}_{1:N}^0-\mathbf{v}^*_{1:N} \right | \le c\mathbf{v}^*_{1:N}$ and  $\mathbf{0}\le\bar{\mathbf{v}}_{N+1:M}^0\le \mathbf{b}$, the $(c\mathbf{v}^*_{1:N},\mathbf{b})$-neighbor coupling
process $\{\bar{\mathbf{v}}^t\}_{t=0}^T$ evolves as:
\begin{enumerate}
    \item Updating state: If $\left | \bar{\mathbf{v}}^t_{1:N}-\mathbf{v}^*_{1:N} \right | \le c\mathbf{v}^*_{1:N}$ and $\mathbf{0}\le \bar{\mathbf{v}}^t_{N+1:M}\le \mathbf{b}$, let $\bar{\mathbf{v}}^{t+1}=\mathbf{v}^{t+1}$,
    \item Absorbing state: Otherwise, maintain $\bar{\mathbf{v}}^{t+1}=\bar{\mathbf{v}}^{t}$.
\end{enumerate}
% The process $\bar{\mathbf{v}}^{t}$ is measurable on $\mathcal{F} ^{t\wedge \tau_{c,\mathbf{b} }}$ where $\tau_{c,\mathbf{b} }=\inf_{t}\left \{ t:\left | \mathbf{v}^t_{1:N}-\mathbf{v}^*_{1:N} \right | >c\mathbf{v}^*_{1:N}\ \vee  \ \mathbf{v}^t_{N+1:M} > \mathbf{b}  \right \} $.
\end{definition}

\subsection{Proof of Phase I}\label{phase 1}\congfang{use restate and subsubsection}

Theorem \ref{theorem_1} establishes that Algorithm \ref{SGD} implicitly selects an optimal truncation dimension $N \in \mathbb{N}_+$ with the following convergence properties:
\begin{enumerate}
    \item For $j \leq N$, $\upv_j^{T_1}$ converges to an adaptive neighborhood of $\upv_j^*$,
    \item For $j > N$, the remaining $\upv_j^{T_1}$ bounded by $\frac{3}{2}\max\{\upv_j^*,2\upv_j^0\}$.
\end{enumerate}  
We construct two critical components: 1) the threshold vector $\hat{\mathbf{v}}^* \in \mathbb{R}^M$ with entries $\hat{\mathbf{v}}_j^* = \max\left\{\frac{3}{2}\mathbf{v}_j^*, 3\mathbf{v}_j^0\right\}$ for any $j \in [1:M]$; 2) the composite vector $\mathbf{b} = ((1 + c_1)(\mathbf{v}_{1:N}^*)^{\top}, (\hat{\mathbf{v}}_{N+1:M}^*)^{\top})^{\top}$, where $c_1 \in (0, 1/2)$.
% Theorem \ref{theorem_1} states that the $T_1$-iteration output of Algorithm \ref{SGD}, initialized at $\mathbf{v}_0$ with a constant step size $\eta$, satisfies the following conditions with high probability:
% 1) For $1 \leq j \leq N$, $\mathbf{v}_j^{T_1}$ converges to $\mathbf{v}_j^{*}$ with an accuracy of $c_1\mathbf{v}_j^{*}$, i.e., $|\mathbf{v}_j^{T_1} - \mathbf{v}_j^{*}| \leq c_1\mathbf{v}_j^{*}$, where $c_1 \in (0, 1/2)$;
% 2) For $N+1 \leq j \leq M$, $\mathbf{v}_j^{T_1}$ remains close to either its initial value $\mathbf{v}_j^{0}$ or $\upv_j^*$. Define $\hat{\mathbf{v}}^* \in \mathbb{R}^M$ as $\hat{\mathbf{v}}_j^* = \max\left\{\frac{3}{2}\mathbf{v}_j^*, 3\mathbf{v}_j^0\right\}$ for any $j \in [M]$. Set $\mathbf{b} = ((1 + c_1)(\mathbf{v}_{1:N}^*)^{\top}, (\hat{\mathbf{v}}_{N+1:M}^*)^{\top})^{\top}$, where $c_1 \in (0, 1/2)$.

\begin{theorem}\label{theorem_1}
	Under Assumption \ref{ass-d}, consider a predictor trained via Algorithm \ref{SGD} with initialization $\mathbf{v}_0$. Let the step size $\eta$ satisfy $\eta \leq \widetilde{\Theta}\left(\frac{c_1^2 \Barsigmin(\max\{N,M\})}{[\sigma^2 + \mathcal{M}^2(\upb)]^2}\right)$ for the optimal truncation dimension $N \in \mathbb{N}_+$ and the scaling constant $c_1 \in (0, 1/2)$. The iteration number $T_1$ requires:
    \begin{align}
        T_1\in\begin{cases}
        \left[\widetilde{\mathcal{O}}\left(\frac{\sigma^2 + \mathcal{M}^2(\upb)}{c_1^2 \eta \sigmin(N)}\right): \widetilde{\Theta}\left(\frac{\Tildesigmax^{-1}(N)}{\eta^2[\sigma^2 + \mathcal{M}^2(\upb)]}\right)\right], \quad &\text{ if }N < M,\notag
        \\
        \left[\widetilde{\mathcal{O}}\left(\frac{\sigma^2 + \mathcal{M}^2(\upb)}{c_1^2 \eta \sigmin(M)}\right):\infty\right), \quad &\text{ otherwise}.
    \end{cases}
    \end{align}
    % When $N < M$, set the iteration number $T_1 \in \left[\widetilde{\mathcal{O}}\left(\frac{\sigma^2 + \mathcal{M}^2(\upb)}{c_1^2 \eta \sigmin(N)}\right), \widetilde{\Theta}\left(\frac{\Tildesigmax^{-1}(N)}{\eta^2[\sigma^2 + \mathcal{M}^2(\upb)]}\right)\right]$. Otherwise, let $T_1 \geq \widetilde{\mathcal{O}}\left(\frac{\sigma^2 + \mathcal{M}^2(\upb)}{c_1^2 \eta \sigmin(M)}\right)$. 
    This configuration guarantees the following convergence property:
    \begin{align}\label{thm-1-eq}
        \begin{cases}
            \upv_j^{T_1}\in\left[\upv_j^{*}-c_1\upv_j^*, \upv_j^{*}+c_1\upv_j^*\right], &\text{ if }j\in[1:N],
            \\
            \upv_j^{T_1}\in\left[0, \frac
            {3}{2}\max\{\upv_j^*,2\upv_j^0\}\right], &\text{ otherwise },
        \end{cases}
    \end{align}
    with probability at least $1-\delta$.
\end{theorem}
We first establish coordinate-wise upper bounds for $\upv^{T_1}$.
\begin{lemma}\label{lemma_1}
Under the setting of Theorem \ref{theorem_1}, let $\{\mathbf{q}^t\}_{t=0}^{T_1}$ be a Markov chain with its $\mathbf{b}$-capped coupling process $\{\bar{\mathbf{v}}^t\}_{t=0}^{T_1}$. When $\eta\leq\widetilde{\Theta}(\frac{1}{\sigma^2+\calM^2(\upb)})$, the inequality $\bar{\upv}^t\geq\textbf{0}$ holds for any $t\in[1:T_1]$. For $\mathbf{v}\in \mathbb{R}^M$, define the truncation event $\calA(\mathbf{v}):=\{\mathbf{v}\leq\mathbf{b}\}$. For $\delta\in(0,1)$, the following conditions guarantee that $\calA(\Bar{\mathbf{v}}^{T_1})$ holds with probability at least $1-\frac{\delta}{6}$:
\begin{enumerate}
    \item Dominant coordinates condition: $\Barsigmin(N)\geq\frac{\eta}{c_1^2}\calO([\sigma^2+\calM^2(\upb)]\log^5(MT_1/\delta))$,
    \item Residual spectrum condition: $\Tildesigmax(N)\geq T_1\eta^2\calO([\sigma^2+\calM^2(\upb)]\log(\max\{M-N,0\}T_1/\delta)$ $\log^4(MT_1/\delta))$.
\end{enumerate}
\end{lemma}
\begin{proof}
Define the random variable 
$$
\mathcal{Z}_j^{t+1}:=\left(\left((\bar{\mathbf{v}}_j^{t})^2-(\mathbf{v}_{j}^{*})^2\right)\hat{\mathbf{x}}_{j}^{t+1}+\hat{\upz}_j^{t+1}(\bar{\upv}^t)-\hat{\zeta}_{M+1:\infty}^{t+1}-\hat{\xi}^{t+1}\right)\hat{\mathbf{x}}_j^{t+1},
$$
for any $j\in[1:M]$ and $t\in[0:T_1-1]$. During the updating state of $\{\bar{\upv}^t\}_{t=0}^{T_1}$, we have
\begin{align}
    \bar{\upv}_j^{t+1}=(1-\eta\calZ_j^{t+1})\bar{\upv}_j^{t},\quad \forall j\in[1:M].
\end{align}
Based on the boundedness of $\mathcal{Z}_j^{t+1}$ and the appropriately chosen step size $\eta\leq\widetilde{\Theta}(\frac{1}{\sigma^2+\calM^2(\upb)})$, if $\bar{\upv}^t>\textbf{0}$, then $\bar{\upv}^{t+1}\geq\frac{1}{2}\bar{\upv}^t$. Since $\bar{\upv}^0>0$,  it follows by induction that $\bar{\upv}^t>0$ for any $t\in[1:T_1]$.
Let $\bar{\tau}_{\mathbf{b} }$ be the earliest time index (mathematically, a stopping time) satisfying $\bar{\mathbf{v}}_j^{\bar{\tau}_{\mathbf{b} }} > \mathbf{b}_j$ for some coordinate $j\in[1:M]$, i.e.,
\begin{equation}\nonumber
      \bar{\tau}_{\mathbf{b} }=\inf_{t}\left \{ t:\exists j\in[1:M], \text{ s.t. }\bar{\mathbf{v}}_j^t > \mathbf{b}_j \right\}.
\end{equation}
For each coordinate $1\le j\le M$, let $\bar{\tau}_{\mathbf{b},j }$ be the earliest time index satisfying $\bar{\mathbf{v}}^{\bar{\tau}_{\mathbf{b},j }}_j > \mathbf{b}_j$, i.e.,
\begin{equation}\nonumber
\bar{\tau}_{\mathbf{b},j }=\inf_{t}\left \{ t:\bar{\mathbf{v}}_j^t > \mathbf{b}_j \right \}.
\end{equation}
Once the stopping time $\bar{\tau}_{\mathbf{b}}=t_2$ occurs for some $t_2\in[1:T_1]$, the coupling process satisfies $\bar{\mathbf{v}}^t=\bar{\mathbf{v}}^{t_2}$ for all $t>t_2$. 

Suppose there exists $j\in[1:N]$ such that $\bar{\tau}_{\mathbf{b},j }=t_2$. 
% Since $\bar{\mathbf{v}}^{t}$ is $\mathcal{F}^t$-measurable, 
Given stopping time $\bar{\tau}_{\mathbf{b},j }=t_2$, the event 
$\mathcal{A} \left ( \bar{\mathbf{v}} ^t \right ) $ holds for all $t\in[0:t_2-1]$. 
% According to Lemma \ref{aux-1}, we establish the sub-Gaussian property for for any $t\in[0:T_1-1]$. Consequently, $\mathcal{Z}_j^{t+1}$ admits high-probability concentration bounds. Given $\bar{\upv}^t$, the iterates admit the recursive bound: $|\bar{\upv}^{t+1}|\leq(1+\widetilde{\calO}(\eta))|\bar{\upv}^t|$ with probability at least $1-\frac{\delta}{12MT_1}$. 
The boundedness of $\mathcal{Z}_j^{t+1}$ and the dominant coordinates condition of $\eta$ imply that  $\bar{\upv}_j^t$ must sequentially enter and exit the threshold interval $[\frac{1}{1+c_1}\mathbf{b}_j,\mathbf{b}_j]$ before exceeding $\upb_j$.
We aim to estimate following probability for coordinates $j\in[1:N]$ and time pairs $t_1<t_2\in[1:T_1]$:
\begin{equation}\nonumber
\bbP\left(\mathcal{B}_{t_1}^{\bar{\tau}_{\mathbf{b},j }=t_2}(j)=\left \{ \bar{\mathbf{v}}_j^{t_1}\leq\frac{1+c_1/2}{1+c_1}\mathbf{
b} _j\wedge \bar{\mathbf{v}}_j^{t_1:t_2-1}\in\left[\frac{1}{1+c_1}\mathbf{b}_j,\mathbf{b}_j\right]\wedge\bar{\mathbf{v}}_j^{t_2}>\mathbf{b}_j  \right \}\right). 
\end{equation}
For any $t\in[t_1:t_2-1]$, we have 
\begin{equation}\label{mar-concen-1}
    \begin{aligned}
        \bbE\left[\bar{\mathbf{v}}_j^{t+1}-\mathbf{v}_j^*\mid\calF^{t}\right]=&\bbE_{\mathbf{x}_{1:M}^{t+1},\xi^{t+1},\zeta_{M+1:\infty}^{t+1}}\left[\bar{\mathbf{v}}_j^{t}-\mathbf{v}_j^*-\eta\calZ_j^{t+1}\bar{\mathbf{v}}_j^{t}\right]
		\\
		\overset{\text{(a)}}{\leq}&\left(1-\frac{1}{2}\eta\lambda_j\bar{\mathbf{v}}_j^{t}(\bar{\mathbf{v}}_j^{t}+\mathbf{v}_j^*)\right)(\bar{\mathbf{v}}_j^{t}-\mathbf{v}_j^*)
		\\
		\leq&\left(1-\frac{1+c_1/2}{\left(1+c_1\right)^2}\eta\lambda_j(\mathbf{v}_j^*)^2\right)(\bar{\mathbf{v}}_j^{t}-\mathbf{v}_j^*),
    \end{aligned}
\end{equation}
where (a) is derived from Assumption \ref{ass-d} and Lemma \ref{aux-1.1}. By applying Lemma \ref{aux-1} to $\mathcal{Z}_j^t$, we demonstrate that $\mathcal{Z}_j^t$ satisfies the sub-Gaussian property for all $t\in[0:T_1-1]$, which yields the bound
\begin{align}
    \bbE\left[\exp\left\{\lambda\left(\bar{\mathbf{v}}_j^{t+1}-\bbE[\bar{\mathbf{v}}_j^{t+1}\mid\calF^t]\right)\right\}\mid\calF^t\right]\leq \exp\left\{\frac{\lambda^2\eta^2\lambda_j(\upv_j^*)^2\calO\left(\left[\sigma^2+\mathcal{M}^2(\upb)\right]\log^4(MT_1/\delta)\right)}{2}\right\},\notag
\end{align}
for any $\lambda\in\bbR$.
% Next, the absolute value of $\bar{\mathbf{v}}_j^{t+1}-\bar{\mathbf{v}}_j^{t}$ over $[t_1:t_2-1]$, can be bounded as follows,
% \begin{equation}\label{bounded-finite-difference}
%     \begin{aligned}
%         \left|\bar{\mathbf{v}}_j^{t+1}-\bar{\mathbf{v}}_j^{t}\right|\leq&\eta\left[\left|\langle\bar{\mathbf{v}}^{t\odot 2}-\mathbf{v}_{1:M}^{*\odot 2},\mathbf{x}_{1:M}^{t}\rangle\right|+\left|\zeta_{M+1:\infty}^t\right|+\left|\xi^{t}\right|\right]\mathbf{x}_j\bar{\mathbf{v}}_j^{t}
% 		\\
%             \leq&\eta\calO\left(\lambda_j^{1/2}\upv_j^*\left(\sigma_{\xi}+\sigma_{\zeta_{M+1:\infty}}+\mathcal{M}^2(\upb)\right)\log(MT_1/\delta)\right)
% 		% \leq&(1+c_1)^2\eta^2\lambda_j(\mathbf{v}_j^*)^2\left[\sigma_{\xi}^2+M(\mathbf{b})\right],
%     \end{aligned}
% \end{equation}
% where the last inequality follows from combining Lemma \ref{aux-1} and the definitions of $\upx_{1:M}$, $\zeta_{M+1:\infty}$ and $\xi$. Notice Eq.~\eqref{bounded-finite-difference} implies that 
% \begin{align}
%     &\left|\bar{\mathbf{v}}_j^{t+1}-\mathbf{v}_j^*-\left(1-\frac{1+c_1/2}{\left(1+c_1\right)^2}\eta\lambda_j(\mathbf{v}_j^*)^2\right)(\bar{\mathbf{v}}_j^{t}-\mathbf{v}_j^*)\right|^2\leq\eta^2\calO\left(\lambda_j(\upv_j^*)^2\left(\sigma^2+\mathcal{M}^2(\upb)\right)\log^2(MT_1/\delta)\right).\notag
% \end{align}
%is derived from the independence between $\mathbf{x}_i$ and $\mathbf{x}_j$ for any $i\neq j$. 
Combining Lemma \ref{aux-2} with Eq.~\eqref{mar-concen-1}, we further establish probability bound for event $\mathcal{B}_{t_1}^{\bar{\tau}_{\mathbf{b},j }=t_2}(j)$ for any time pair $t_1<t_2\in[1:T_1]$.
\begin{align}\label{probability-1}
\Pro\left(\mathcal{B}_{t_1}^{\bar{\tau}_{\mathbf{b},j }=t_2}(j)\right )\leq&\exp\left\{-\frac{c_1^2(\mathbf{v}_j^*)^2}{\eta\calO\left([\sigma^2+\mathcal{M}^2(\upb)]\log^4(MT_1/\delta)\right)}\right\}.
\end{align}
	
Suppose there exists $j\in[N+1:M]$ such that $\bar{\tau}_{\mathbf{b},j }=t_2$. Given stopping time $\bar{\tau}_{\mathbf{b},j }=t_2$, the event 
$\mathcal{A} \left ( \bar{\mathbf{v}} ^t \right ) $ holds for all $t\in[0:t_2-1]$. Similarly, $\bar{\upv}_j^t$ must sequentially enter and exit the threshold interval $[\frac{2}{3}\upb_j,\upb_j]$ before exceeding $\upb_j$. Therefore, we aim to estimate following probability for coordinates $j\in[N+1:M]$ and time pairs $t_1<t_2\in[1:T_1]$:
\begin{equation}\nonumber
    \bbP\left(\calC_{t_1}^{\bar{\tau}_{\mathbf{b},j }=t_2}(j)=\left\{\bar{\mathbf{v}}_j^{t_1}\leq\frac{3}{4}\mathbf{b}_j\bigwedge\bar{\mathbf{v}}_j^{t_1:t_2-1}\in\left[\frac{2}{3}\upb_j,\mathbf{b}_j\right]\bigwedge \bar{\mathbf{v}}_j^{t_2}>\mathbf{b}_j \right\}\right).
\end{equation}
For any $t\in[t_1:t_2-1]$, we have 
\begin{equation}\label{mar-concen-2}
    \begin{aligned}
         \bbE\left[\bar{\mathbf{v}}_j^{t+1}-\mathbf{v}_j^*\mid\calF^{t}\right]=&\bbE_{\mathbf{x}_{1:M}^{t+1},\xi^{t+1},\zeta_{M+1:\infty}^{t+1}}\left[\bar{\mathbf{v}}_j^{t}-\mathbf{v}_j^*-\eta\calZ_j^{t+1}\bar{\mathbf{v}}_j^{t}\right]
		\\
		\leq&\left(1-\frac{1}{2}\eta\lambda_j\bar{\mathbf{v}}_j^{t}(\bar{\mathbf{v}}_j^{t}+\mathbf{v}_j^*)\right)(\bar{\mathbf{v}}_j^{t}-\mathbf{v}_j^*)
		\\
		\leq &\bar{\mathbf{v}}_j^{t}-\mathbf{v}_j^*.
    \end{aligned}
\end{equation}
Similarly, using Lemma \ref{aux-1}, we have
\begin{align}
    \bbE\left[\exp\left\{\lambda(\bar{\upv}_j^{t+1}-\bbE[\bar{\upv}_j^{t+1}\mid\calF^t])\right\}\mid\calF^t\right]\leq\exp\left\{\frac{\lambda^2\eta^2\lambda_j(\upb_j^*)^2\calO\left(\left[\sigma^2+\mathcal{M}^2(\upb)\right]\log^4(MT_1/\delta)\right)}{2}\right\},\notag
\end{align}
for any $\lambda\in\bbR$. Combining Lemma \ref{aux-2} with Eq.~\eqref{mar-concen-2}, we further establish probability bound for event $\mathcal{C}_{t_1}^{\bar{\tau}_{\mathbf{b},j }=t_2}(j)$ for any time pair $t_1<t_2\in[1:T_1]$.
	\begin{align}\label{probability-2}
		\Pro\left (\calC_{t_1}^{\bar{\tau}_{\mathbf{b},j }=t_2}(j)\right )\leq\exp\left\{-\frac{1}{T\eta^2\lambda_j\calO\left([\sigma^2+\calM^2(\upb)]\log^2(MT_1/\delta)\right)}\right\}.
	\end{align}
% Finally, we can obtain the following probability bound of event $(\calA(\bar{\mathbf{v}}^{T_1}))^c$ with above probability bounds Eq.~\eqref{probability-1} and Eq.\eqref{probability-2}, and dominant coordinates condition and residual spectrum condition:
Ultimately, combining the probability bounds Eq.~\eqref{probability-1} and Eq.\eqref{probability-2} with the dominant coordinates condition and residual spectrum condition, we obtain the following probability bound for complement event $\calA^c(\bar{\mathbf{v}}^{T_1})$:
	\begin{align}\label{union-1}
		\Pro\left(\calA^c(\bar{\mathbf{v}}^{T_1})\right ) \leq&\sum_{j=1}^N\sum_{1\leq t_1<t_2\leq T_1}\Pro\left(\mathcal{B}_{t_1}^{\bar{\tau}_{\mathbf{b},j }=t_2}(j)\right)\notag+\sum_{j=N+1}^M\sum_{1\leq t_1<t_2\leq T_1}\Pro\left(\calC_{t_1}^{\bar{\tau}_{\mathbf{b},j }=t_2}(j)\right) \notag
		\\
		\leq&\frac{NT_1^2}{2}\exp\left\{-\frac{c_1^2\min_{1\le j\le N}(\mathbf{v}_j^*)^2}{\eta\calO\left(\left[\sigma^2+\calM^2(\upb)\right]\log^4(MT_1/\delta)\right)}\right\}\notag
		\\
		&+\max\{M-N,0\}T_1\exp\left\{-\frac{\min_{N+1\le j\le M}\lambda_j^{-1}}{T_1\eta^2\calO\left([\sigma^2+\calM^2(\upb)]\log^4(MT_1/\delta)\right)}\right\}\notag
		\\
		\leq&\frac{\delta}{12}.
	\end{align}
\end{proof}

Lemma \ref{lemma_1} establishes the adaptive high-probability upper bounds for each component of $\bar{\upv}^{T_1}$. According to the construction methodology of the coupling process $\{\bar{\upv}^t\}_{t=0}^{T_1}$, these bounds naturally extends to $\upq^{T_1}$. Moreover, the high-probability consistency between control sequence $\{\upq^t\}_{t=0}^{T}$ and original sequence $\{\upv^t\}_{t=0}^{T}$ (established in Proposition \ref{p1}) allows direct verification that Lemma \ref{lemma_1}'s result applies to $\upv^{T_1}$. Consequently, Lemmas \ref{lemma-2} and \ref{lemma-3} remain valid for sequence $\{\upv^t\}_{t=0}^{T_1}$ under this logical framework.

Deriving a direct high-probability lower bound for $\bar{\upv}^{T_1}$ proves challenging. Therefore, we apply Lemma \ref{lemma-2} to construct such bounds for $\max_{t\in[1:T_1]}\bar{\upv}_j^t$ adaptively over $j\in[1:N]$.
\begin{lemma}\label{lemma-2}
	Under the setting of Lemma \ref{lemma_1}, let  $\eta\leq\frac{c_1\log^{-4}(MT_1/\delta)\min_{j\in[1:N]}(\upv_j^*)^2}{\calO(\sigma^2+(1+C)\mathcal{M}^2(\upb))}$ and 
    $$
    T_1\geq\max\left\{\frac{\calO\left(\max_{j\in[1:N]}-\log(\upv_j^0)\right)}{c_1\eta\sigmin(N)},\frac{\calO\left([\sigma^2+\mathcal{M}^2(\upb)]\log^8(MT_1/\delta)\right)}{c_1^2\min_{j\in[1:N]}(\lambda_j(\upv_j^*)^4)}\right\}.
    $$
    The combined event set satisfies $\mathbb{P}\left(\left(\bigcap_{j=1}^N\calE_{1,j}\right)\bigcup\calE_2\right) \geq 1 - \frac{\delta}{6}$. These events are defined as:
    % one of the following cases holds with probability at least $1-\frac{\delta}{6N}$:
	\begin{enumerate}
		\item[\textbf{[$\calE_{1,j}$]}] $\max_{t\leq T_1}\bar{\upv}_j^t\geq\frac{1-c_1/2}{1+c_1}\upb_j$,
		\item[\textbf{[$\calE_2$]}] $\calA^c(\bar{\upv}^{T_1})$.
	\end{enumerate}
\end{lemma}
\begin{proof}
    For a fixed $j\in[1:N]$, we define 
    % $Y_j^t:=\llangle\bar{\upv}^{t\odot 2}-\upv_{1:M}^{*\odot 2},\upx_{1:M}^{t}\rrangle-\left((\bar{\upv}_j^t)^2-(\upv_j^*)^2\right)\upx_j^t-\zeta_{M+1:\infty}^t-\xi^{t}$ for any $t\in[0:T_1-1]$ and 
    another coupling $\{\breve{\upv}^t\}_{t=0}^{T_1}$ with initialization $\breve{\upv}^0=\bar{\upv}^0$ as follows: 
    \begin{enumerate}
        \item Updating state: If 
        % $|Y_j^t|\leq R_j:=\calO\left([\sigma^2+\mathcal{M}^2(\upb)]^{1/2}\log^2(MT_1/\delta)R\right)$ and the 
        event $\calB_t(j)=\left\{\calA(\breve{\upv}^t)\bigwedge\breve{\upv}_j^t<\frac{1-c_1/2}{1+c_1}\upb_j\right\}$ holds, let $\breve{\upv}^{t+1}=\bar{\upv}^{t+1}$,
        \item Multiplicative scaling state: Otherwise, let $\breve{\upv}^{t+1}=\left(1+\frac{c_1(1-c_1)\eta}{2}\lambda_{j}(\upv_{j}^*)^2\right)\breve{\upv}^{t}$.
    \end{enumerate}
    Next, we aim to show that $-t\log(1+\frac{c_1(1-c_1)\eta}{2}\lambda_{j}(\upv_{j}^*)^2)+\log(\breve{\upv}_j^t)$ is a submartingale. 
    If event $\calB_t^c(j)$ holds, we directly obtain $\bbE[\log(\breve{\upv}_j^{t+1}) \mid \calF^t] \geq \log(1+\frac{c_1(1-c_1)\eta}{2}\lambda_j(\upv_j^*)^2) + \log(\breve{\upv}_j^t)$. Otherwise, letting 
    $$
    \calY_j^t:=\hat{z}_j^t(\bar{\upv}^{t-1})-\hat{\zeta}_{M+1:\infty}^t-\hat{\xi}^t,\quad \forall t\in[1:T_1],
    $$ 
    we have
    % If event $\calB_t^c(j)$ occurs or $Y_j^t$ escapes from $\calB_{R_j}(0)$, it is straightforward to obtain $\bbE\left[\log(\breve{\upv}_j^{t+1})\mid\calF^t\right]\geq\log\left(1+\frac{c_1(1-c_1)\eta}{2}\lambda_{j}(\upv_{j}^*)^2\right)+\log(\breve{\upv}_j^t)$. Otherwise, we have
	\begin{align}
		\bbE\left[\log(\breve{\upv}_j^{t+1})\mid\calF^t\right]=&\bbE\left[\log(\bar{\upv}_j^{t+1})\mid\calF^t\right]\notag
		\\
		=&\bbE_{\upx_{1:M}^{t+1},\xi^{t+1},\zeta_{M+1:\infty}^{t+1}}\left[\log\left(1-\eta\left((\bar{\upv}_j^t)^2-(\upv_j^*)^2\right)(\hat{\upx}_j^{t+1})^2-\eta \calY_j^{t+1}\hat{\upx}_j^{t+1}\right)\right]\notag
        \\
        &+\log(\bar{\upv}_j^t)\notag
	\\
	\overset{\text{(a)}}       {\geq}&\log\left(1+\frac{3c_1(1-c_1)\eta}{4}\lambda_j(\upv_j^*)^2\right)\notag
        \\
        &-\eta^2\lambda_j\calO\left(\left[\sigma^2+(1+C)\mathcal{M}^2(\upb)\right]\log^4(MT_1/\delta)\right)+\log(\bar{\upv}_j^t)\notag
        \\
        \overset{\text{(b)}}{\geq}&\log\left(1+\frac{c_1(1-c_1)\eta}{2}\lambda_j(\upv_j^*)^2\right)+\log(\bar{\upv}_j^t)\notag
		\\
		\overset{\text{(c)}}{=}&\log\left(1+\frac{c_1(1-c_1)\eta}{2}\lambda_j(\upv_j^*)^2\right)+\log(\breve{\upv}_j^t),\notag
	\end{align} 
    where (a) originates from three components: 1) the Taylor expansion of $\log(a+\cdot)$ for $a=1+\eta((\upv_j^*)^2-(\bar{\upv}_j^t)^2)\bbE[(\hat{\upx}_j^{t+1})^2]$; 2) the property that $Y_j^{t+1}$ has zero mean and is independent of $\hat{\upx}_j^{t+1}$, and 3) the step size setting $\eta\leq\frac{c_1(\upv_j^*)^2\log^{-4}(MT_1/\delta)}{\calO(\sigma^2+(1+C)\mathcal{M}^2(\upb))}$ ensures that $1-\tau\eta((\bar{\upv}_j^t)^2-(\upv_j^*)^2)[(\hat{\upx}_j^{t+1})^2-\bbE[(\hat{\upx}_j^{t+1})^2]]-\tau\eta \calY_j^{t+1}\hat{\upx}_j^{t+1}\geq1/2$ for any $\tau\in[0,1]$, 
    (b) is drawn from the inequality $\log(1+\frac{c_1(1-c_1)\eta}{16}\lambda_j(\upv_j^*)^2)\geq\eta^2\lambda_j\calO([\sigma^2+(1+C)\mathcal{M}^2(\upb)]$ $\log^4(MT_1/\delta))$, and (c) relies on the temporal exclusivity property: if event $\calB_t^c(j)$ occurs at time $t$, then $\calB_{t}(j)$ is permanently excluded for all subsequent times $t' > t$. Therefore, we obtain
    \begin{align}\label{lower-2}
        &\Pro\left\{\breve{\upv}_j^{T_1}<\frac{1-c_1/2}{1+c_1}\upb_j\right\}\notag
        \\
        \overset{\text{(d)}}{\leq}&\exp\left\{-\frac{2\left({T_1}\log\left(1+\frac{c_1(1-c_1)\eta}{2}\lambda_j(\upv_j^*)^2\right)+\log(v_j^0)-\log\left(\frac{1-c_1/2}{1+c_1}\upb_j\right)\right)^2}{{T_1}\eta^2\lambda_j\calO\left([\sigma^2+\mathcal{M}^2(\upb)]\log^6(MT_1/\delta)\right)}\right\}\notag
        \\
        \overset{\text{(e)}}{\leq}&\exp\left\{-\frac{{T_1}\log^2\left(1+\frac{c_1(1-c_1)\eta}{2}\lambda_j(\upv_j^*)^2\right)}{\eta^2\lambda_j\calO\left([\sigma^2+\mathcal{M}^2(\upb)]\log^6(MT_1/\delta)\right)}\right\}\notag
        \\
        \overset{\text{(f)}}{\leq}&\frac{\delta}{12N}
    \end{align}
    where (d) is derived from Azuma's inequality and the estimation of $\left|\log(\breve{\upv}_j^{t+1})-\log(\breve{\upv}_j^{t})\right|$ as follows:
    \begin{align}
        \left|\log(\breve{\upv}_j^{t+1})-\log(\breve{\upv}_j^{t})\right|\leq\eta\lambda_j^{1/2}\calO\left(\left[\sigma^2+\mathcal{M}^2(\upb)\right]^{1/2}\log^4(MT_1/\delta)\right),
    \end{align}
    which implies that
    \begin{align}
        \left|\log(\breve{\upv}_j^{t+1})-\log\left(1+\frac{c_1(1-c_1)\eta}{2}\lambda_{j}(\upv_{j}^*)^2\right)-\log(\breve{\upv}_j^{t})\right|^2\leq\eta^2\lambda_j\calO\left([\sigma^2+\mathcal{M}^2(\upb)]\log^8(MT_1/\delta)\right).\notag
    \end{align}
    Moreover, since ${T_1}\log(1+\frac{c_1(1-c_1)\eta}{2}\lambda_j(\upv_j^*)^2)/4\geq-\log(v_j^0)$ and $c_1^2{T_1}\lambda_j(\upv_j^*)^4\geq\calO([\sigma^2+\mathcal{M}^2(\upb)]$ $\log^8(MT_1/\delta))$, we obtain inequality (e) and (f). 
    % By combining Lemma \ref{aux-1} and the properties of sub-Gaussian variables, we have $|Y_j^t|>R_j$ with a probability of at most $\frac{\delta}{12MT_1}$ for any $t\in[0:T_1-1]$. 
    If $\calA(\bar{\upv}^{T_1})$ holds, Eq.~\eqref{lower-2} implicates that $\bbP(\calE_{1,j}^c)\leq\frac{\delta}{12N}$. Thus, we have $\bbP(\calE_{1,j}^c\bigcap\calE_2^c)\leq\frac{\delta}{6N}$.
\end{proof}

Lemma~\ref{lemma-3} establishes a high-probability lower bound for $\bar{\mathbf{v}}_j^{T_1}$ for any $j\in[1:N]$. This constitutes the final component required to complete Theorem \ref{theorem_1}.

\begin{lemma}\label{lemma-3}
    Under the setting of Lemma \ref{lemma_1}, let $\eta\leq\frac{c_1^2\Barsigmin(N)}{\calO([\sigma^2+\calM^2(\upb)]\log^4(MT_1/\delta))}$. The combined event set satisfies $\mathbb{P}\left(\bigcap_{j=1}^N\left(\bigcup_{k={3,4}}\calE_{k,j}\right)\right) \geq 1 - \frac{\delta}{6}$. These events are defined as:
	\begin{enumerate}
		\item[\textbf{[$\calE_{3,j}$]}] $\max_{t\leq T_1}\bar{\mathbf{v}}_j^t<\frac{1-c_1/2}{1+c_1}\mathbf{b}_j$,
		\item[\textbf{[$\calE_{4,j}$]}] $\bar{\mathbf{v}}_j^{T_1}\geq\frac{1-c_1}{1+c_1}\mathbf{b}_j$.
	\end{enumerate}
\end{lemma}
\begin{proof}
For any $j \in [1:N]$, if $\mathcal{E}_{3,j}^c$ occurs, there exists $t \in [1:T_1]$ satisfying $\bar{\mathbf{v}}_j^t \geq \frac{1 - c_1/2}{1 + c_1}\mathbf{b}_j$. 
Define $\tau_{0,j}$ as the earliest time index satisfying $\bar{\mathbf{v}}_j^{\tau_{0,j}} \geq \frac{1 - c_1/2}{1 + c_1}\mathbf{b}_j$:
\begin{equation}\nonumber
   \tau_{0,j}=\inf_{t}\left \{ t:\bar{\mathbf{v}}_j^{t}\ge \frac{1-c_1/2}{1+c_1}\mathbf{b}_j\right \}.
\end{equation}
Then, we define $\tau_{1,j}$ as the earliest time index satisfying $\bar{\mathbf{v}}_j^{\tau_{1,j}}<\frac{1-c_1}{1+c_1}\mathbf{b}_j$ after $\tau_{0,j}$:
\begin{equation}\nonumber
     \tau_{1,j} =\inf_{t>\tau_{0,j}}\left \{ t:\bar{\mathbf{v}}_j^{t}<\frac{1-c_1}{1+c_1}\mathbf{b}_j\right \}.
\end{equation}
By the definition of $\{\bar{\mathbf{v}}^t\}_{t=0}^{T_1}$, once the event $\calA^c(\bar{\mathbf{v}}^t)$ occurs, the coupling process satisfies $\bar{\mathbf{v}}^{t'}=\bar{\mathbf{v}}^{t}$ for any $t'>t$. Therefore, $\mathcal{A}(\bar{\mathbf{v}}^t)$ holds for all $t \leq \tau_{1,j}$. Similarly, $\bar{\upv}_j^t$ must sequentially enter and exit the threshold interval $[\frac{1-c_1}{1+c_1}\upb_j,\frac{1}{1+c_1}\upb_j]$ before subceeding $\frac{1-c_1}{1+c_1}\upb_j$. We aim to estimate following probability for coordinates $j\in[1:N]$ and time pairs $t_0<t_1\in[1:T_1]$:
% For any $1\le t_0<t_1\le T_1$,  we next bound the probability of the event
\begin{equation}\nonumber
    \bbP\left(\bar{\mathcal{D} }_{\tau_0=t_0}^{\tau_1=t_1}\left ( j \right )=\left\{\bar{\mathbf{v}}_j^{t_0}\geq\frac{1-c_1/2}{1+c_1}\mathbf{b}_j\bigwedge\bar{\mathbf{v}}_j^{t_0:t_1-1}\in\left[\frac{1-c_1}{1+c_1}\mathbf{b}_j,\frac{1}{1+c_1}\mathbf{b}_j\right]\bigwedge\bar{\mathbf{v}}_j^{t_1}<\frac{1-c_1}{1+c_1}\mathbf{b}_j\right\}\right).
\end{equation}
% For any $t_0\le t<t_1$, let $\mathcal{F}^t$ denote the $\sigma$-algebra generated by $\{\bar{\mathbf{v}}^i\}_{i=0}^t$. 
For any $t\in[t_0:t_1-1]$, we have 
\begin{equation}\label{mar-concen-3}
    \begin{aligned}
        \bbE\left[\mathbf{v}_j^*-\bar{\mathbf{v}}_j^{t+1}\mid\mathcal{F}^t\right]=&\bbE_{{\mathbf{x}}_{1:M}^{t+1},{\xi}^{t+1},{\zeta}_{M+1:\infty}^{t+1}}\left[\mathbf{v}_j^*-\bar{\mathbf{v}}_j^{t}+\eta\left(\left((\bar{\upv}_j^t)^2-(\upv_j^*)^2\right)\hat{\upx}_j^{t+1}+\hat{\upz}_j^{t+1}(\bar{\upv}^t)\right.\right.
        \\
        &\, \, \, \, \, \, \, \, \, \, \, \, \, \, \, \, \, \, \, \, \, \, \, \, \, \, \, \, \, \, \, \, \, \, \, \, \, \, \, \, \, \, \, \, \, \left.\left.-\hat{\zeta}_{M+1:\infty}^{t+1}-\hat{\xi}^{t+1}\right)\hat{\mathbf{x}}_j^{t+1}\bar{\mathbf{v}}_j^{t+1}\right]
		% \\
		% =&(1-\eta\lambda_j\bar{\mathbf{v}}_j^{t}(\bar{\mathbf{v}}_j^{t}+\mathbf{v}_j^*))(\mathbf{v}_j^*-\bar{\mathbf{v}}_j^{t})\notag
		\\
		\leq&\left(1-\frac{1-c_1}{(1+c_1)^2}\eta\lambda_{j}(\mathbf{v}_{j}^*)^2\right)(\mathbf{v}_j^*-\bar{\mathbf{v}}_j^{t}).
    \end{aligned}
\end{equation}
Applying Lemma \ref{aux-1} to $(((\bar{\upv}_j^t)^2-(\upv_j^*)^2)\hat{\upx}_j^{t+1}+\hat{\upz}_j^{t+1}(\bar{\upv}^t)-\hat{\zeta}_{M+1:\infty}^{t+1}-\hat{\xi}^{t+1})\hat{\mathbf{x}}_j^{t+1}$, we have
\begin{align}
    \bbE\left[\exp\left\{\lambda\left(\bbE[\bar{\mathbf{v}}_j^{t+1}\mid\calF^t]-\bar{\mathbf{v}}_j^{t+1}\right)\right\}\mid\calF^t\right]\leq \exp\left\{\frac{\lambda^2\eta^2\lambda_j(\upv_j^*)^2\calO\left(\left[\sigma^2+\mathcal{M}^2(\upb)\right]\log^4(MT_1/\delta)\right)}{2}\right\},\notag
\end{align}
for any $\lambda\in\bbR$. Therefore, combining Lemma \ref{aux-2} with Eq.~\eqref{mar-concen-3}, we further establish the probability bound for event $\bar{\mathcal{D} }_{\tau_0=t_0}^{\tau_1=t_1}\left(j\right)$ for any time pair $t_0<t_1\in[1:T_1]$, 
	\begin{align}\nonumber
		\Pro\left(\bar{\mathcal{D} }_{\tau_0=t_0}^{\tau_1=t_1}\left ( j \right )\right)\leq\exp\left\{\frac{-c_1^2(\mathbf{v}_j^*)^2}{\eta\calO\left(\left[\sigma^2+\calM^2(\upb)\right]\log^4(MT_1/\delta)\right)}\right\}.
	\end{align}
 Notice that the occurrence of  $\calE_{3,j}^c\bigwedge\calE_{4,j}^c$ implies $\bar{\mathcal{D} }_{\tau_0=t_0}^{\tau_1=t_1}\left ( j \right )$  must hold for some $t_0<t_1\in[1:T_1]$. Therefore, we have
	\begin{align}
		\Pro\left(\calE_{3,j}^c\wedge\calE_{4,j}^c\right)\leq&\sum_{1\leq t_1<t_2\leq T_1}	\Pro\left(\bar{\mathcal{D} }_{\tau_0=t_0}^{\tau_1=t_1}\left ( j \right )\right)\notag
		\\
		\leq&\frac{T_1^2}{2}\exp\left\{\frac{-c_1^2(\mathbf{v}_j^*)^2}{\eta\calO\left(\left[\sigma^2+\calM^2(\upb)\right]\log^4(MT_1/\delta)\right)}\right\}\notag
		\\
		\leq&\frac{T_1^2}{2}\exp\left\{\frac{-c_1^2\min_{j\in[1:N]}(\mathbf{v}_{j}^*)^2}{\eta\calO\left(\left[\sigma^2+\calM^2(\upb)\right]\log^4(MT_1/\delta)\right)}\right\}\notag
		\\
		\leq&\frac{\delta}{6N}.
	\end{align}

\end{proof}

We are now prepared to prove Theorem \ref{theorem_1}.

\begin{proof}[Proof of Theorem \ref{theorem_1}]
	% Given the step size $\eta$ and sampling number $T_1$, it is necessary to ensure that the conditions in Lemma \ref{lemma_1}--Lemma \ref{lemma-3} are all satisfied. 
    Notice that
	\begin{align}\label{eta-choice}
		\eta\leq\frac{c_1^2\Barsigmin(N)}{\calO\left(\left[\sigma^2+\mathcal{M}^2(\upb)\right]\log^4(MT_1/\delta)\right)},
	\end{align} 
	and  
	\begin{align}\label{T-choice}
		\begin{cases}
			\frac{\calO\left([\sigma^2+\mathcal{M}^2(\upb)]\log^8(MT_1/\delta)-\min_{j\in[1:N]}\log(\upv_j^0)\right)}{c_1^2\eta\sigmin(N)}\leq T_1\leq\frac{\log^{-4}(MT_1/\delta)\log((M-N)T_1/\delta)}{\eta^2\Tildesigmax(N)\calO\left([\sigma^2+\mathcal{M}^2(\upb)]\right)}, & \text{ if }M>N,
			\\
			\frac{\calO\left([\sigma^2+\mathcal{M}^2(\upb)]\log^8(MT_1/\delta)-\min_{j\in[1:N]}\log(\upv_j^0)\right)}{c_1^2\eta\sigmin(N)}\leq T_1, & \text{ otherwise }.
		\end{cases}
	\end{align}
	Then, Eq.~\eqref{eta-choice} and Eq.~\eqref{T-choice} can be verified to satisfy all assumptions in Lemmas \ref{lemma_1}-\ref{lemma-3}.

	Lemma \ref{lemma_1} yields $\Pro\{\bar{\upv}^{T_1}>\upb\}\leq\frac{\delta}{6}$. Lemma \ref{lemma-2} implies that $\Pro\{\min_{j\in[1:N]}\max_{t\leq {T_1}}(\bar{\upv}_j^t-\frac{1-c_1/2}{1+c_1}\upb_j)<0\bigwedge\bar{\upv}^{T_1}\leq\upb\}\leq\frac{\delta}{6}$. Therefore, combining Lemma \ref{lemma_1} and \ref{lemma-2}, we have $\Pro\{\min_{j\in[1:N]}$ $\max_{t\leq {T_1}}(\bar{\upv}_j^t-\frac{1-c_1/2}{1+c_1}\upb_j)<0\}\leq\frac{\delta}{3}$. Moreover, Lemma \ref{lemma-3} implicates that $\Pro\{\min_{j\in[1:N]}$ $\max_{t\leq {T_1}}(\bar{\upv}_j^t-\frac{1-c_1/2}{1+c_1}\upb_j)\geq0\bigwedge\min_{j\in[1:N]}(\bar{\upv}_j^{T_1}-\frac{1-c_1}{1+c_1}\upb_j)<0\}\leq\frac{\delta}{6}$. Combining these results establishes the final probability bound: $\Pro\{|\bar{\upv}_{1:N}^{T_1}-\upv_{1:N}^*|\leq\frac{c_1}{1+c_1}\upb_{1:N}\bigwedge\bar{\upv}_{N+1:M}^{T_1}\leq\upb_{N+1:M}\}\geq1-\frac{2}{3}\delta$, and this bound can be extended to $\upq^{T_1}$. By Proposition \ref{p1}, we complete the proof.
\end{proof}

\subsection{Proof of Phase II}\label{phase-2}

In this phase, we first demonstrate that after Phase I (i.e., $t>T_1$), the iterations of $\upv^t$ are, with high probability, confined within a neighborhood of $\upv_{1:M}^*$. Next, we show that when the iterations of $\upv^t$ are constrained to a neighborhood of $\upv_{1:M}^*$, the dynamics of SGD for the quadratic model approximate those of SGD for the linear model. Therefore, we can apply the analytical techniques for SGD in the linear model to derive the conclusion of Theorem \ref{theorem-3}. To meet the requirements of the analysis in Phase II, 
we introduce the truncated coupling $\{\widehat{\upv}^t\}_{t=0}^{T_2}$ as follows:
\begin{align}
	\widehat{\upv}^{t+1}=\begin{cases}
		% \frac{1}{4}\upv_{1:M}^*, & \text{ if }\exists j\in[1:N],\, \widehat{\upv}_j^t<\frac{1}{2}\upv_j^*,
  %       \\
		\upv^{T_1+t+1}, & \text{ if }\forall j\in[1:N],\, \widehat{\upv}_j^t\in[\frac{1}{2}\upv_j^*,\frac{3}{2}\upv_j^*]\text{ and }\forall j\in[N+1:M],\, \widehat{\upv}_j^t\in[0,2\upv_j^*],
		\\
		\frac{13}{4}\upv_{1:M}^*, & \text{ otherwise },\notag
        % \text{ if }\exists j\in[1:N],\, \widehat{\upv}_j^t>\frac{3}{2}\upv_j^*\text{ or }\exists j\in[N+1:M],\, \widehat{\upv}_j^t>2\upv_j^*,\notag
	\end{cases}
\end{align}
with initialization $\widehat{\upv}^0=\upv^{T_1}$. In addition, we define the auxiliary function $\psi:\bbR^M\rightarrow\bbR^M$:
\begin{align}
	\psi(\upv)=\begin{cases}
		\upv, & \text{ if }\forall j\in[1:N],\, \upv_j\in[\frac{1}{2}\upv_j^*,\frac{3}{2}\upv_j^*]\text{ and }\forall j\in[N+1:M],\, \upv_j\in[0,2\upv_j^*],
		\\
		\upv_{1:M}^*, & \text{ otherwise}.
	\end{cases}\notag
\end{align}
In phase II, we consider the discrete dynamic of $\upw^t=\psi(\widehat{\upv}^{t})$ for any $t\in[0:T_2]$.

\noindent\textbf{Preliminary: }For any vectors $\upv,\upu\in\bbR^d$, we define $\upv\odot\upu=(\upv_1\upu_1,\cdots,\upv_d\upu_d)^{\top}$ and $\diag\{\upv\}=\diag\{\upv_1,\cdots,\upv_d\}\in\bbR^{d\times d}$. We also denote for simplicity $\upH_{\upw}^t=(\upw^t\odot\Pi_M\upx^t)\otimes((\upw^t+\upv_{1:M}^*)\odot$ $\Pi_M\upx^t)$ and $\upR_{\upw}^t=(\xi^t+\zeta_{M+1:\infty}^t)\diag\{\upw^t\}$.
We now summarize the linear operators that will be used in the proof:
\begin{align}
	\calI:=\upI\otimes\upI,\quad &\calH_{\upw}^t:=\bbE_t\left[\upH_{\upw}^t\otimes(\upH_{\upw}^t)^{\top}\right],\quad \widetilde{\calH}_{\upw}^t:=\bbE_t\left[\upH_{\upw}^t\right]\otimes\bbE_t\left[\upH_{\upw}^t\right],\notag
	\\
	\calG_{\upw}^t:=\bbE_t\left[\upH_{\upw}^t\right]\otimes\upI+\upI\otimes&\bbE_t\left[\upH_{\upw}^t\right]-\eta_t\calH_{\upw}^t,\quad \widetilde{\calG}_{\upw}^t:=\bbE_t\left[\upH_{\upw}^t\right]\otimes\upI+\upI\otimes\bbE_t\left[\upH_{\upw}^t\right]-\eta_t\widetilde{\calH}_{\upw}^t.\notag
\end{align}
For any operator $\calA$, we use the notation $\calA\circ\upA$ to denote $\calA$ acting on a symmetric matrix $\upA$. It's also direct to verify the following rules for above operators acting on a symmetric matrix $\upA$:
\begin{align}
	\calI\circ\upA=\upA,\quad \calH_{\upw}^t\circ\upA=&\bbE\left[\upH_{\upw}^t\upA(\upH_{\upw}^t)^{\top}\right],\quad\widetilde{\calH}_{\upw}^t\circ\upA=\bbE\left[\upH_{\upw}^t\right]\upA\bbE\left[\upH_{\upw}^t\right],\notag
	\\
	\left(\calI-\eta_t\calG_{\upw}^t\right)\circ\upA=&\bbE\left[\left(\upI-\eta_t\upH_{\upw}^t\right)\upA\left(\upI-\eta_t\upH_{\upw}^t\right)\right],\notag
	\\
	\left(\calI-\eta_t\widetilde{\calG}_{\upw}^t\right)\circ\upA=&\left(\upI-\eta_t\bbE\left[\upH_{\upw}^t\right]\right)\upA\left(\upI-\eta_t\bbE\left[\upH_{\upw}^t\right]\right).\notag
\end{align}
Notice Theorem \ref{theorem_1} guarantee that algorithmic output after $T_1$ iterations approximates the ground truth within a constant factor, namely, $|\upv_{1:N}-\upv_{1:N}^*|\leq c_1\upv_{1:N}^*$. In this phase, we will use $\upv^{T_1}$, which satisfies Eq.~\eqref{thm-1-eq}, as the initial point for the SGD iterations and anneal the learning rate to guarantee the function value at the algorithm's output fully converges to $\calR_M(\upv_{1:M}^*)$. 
\begin{lemma}\label{high-probability-phase-II}
Under Assumption \ref{ass-d}, we consider the $T_1$-th step of Algorithm \ref{SGD} and its subsequent iterative process. Let $N \in \mathbb{N}+$ represent the optimal truncation dimension. Define $\eta_0 \leq \widetilde{\Theta}\left(\frac{\Barsigmin(\max\{N,M\})}{\sigma^2 + \calM^2(\upb)}\right)$, and let $\{\widetilde{\upv}^t\}_{t=0}^{T_2}$ be a $(1/2,2)$-$\upv^*$ neighbor coupling process based on the control sequence $\{\upq^{T_1+t}\}_{t=0}^{T_2}$. We denote the event $\calG(\upv):=\{|\upv_{1:N}-\upv_{1:N}^*|\leq\frac{1}{2}\upv_{1:N}^*\bigwedge\boldsymbol{0}_{N+1:M}\leq\upv_{N+1:M}\leq2\upv_{N+1:M}^*\}$ for any $\upv\in\bbR^M$. If $N < M$, set the iteration number $T_2 \in \left[1: \widetilde{\Theta}\left(\frac{\Tildesigmax^{-1}(N)}{\eta_0^2 [\sigma^2 + \calM^2(\upb)]}\right)\right]$. Otherwise, let $T_2$ be an arbitrary positive integer. Then, with probability at least $1 - \delta$, we have $\bigcap_{t=0}^{T_2}\calG(\upv^{T_1+t})$ holding.
\end{lemma}
\begin{proof}
	Setting $c_1=\frac{1}{4}$ in Theorem \ref{theorem_1} yields with probability at least $1-\delta/6$: $|\upq_{1:N}^{T_1}-\upv_{1:N}^*|\leq\frac{1}{4}\upv_{1:N}^*$ and $\boldsymbol{0}_{N+1:M}\leq\upq_{N+1:M}^{T_1}\leq\frac{3}{2}\upv_{N+1:M}^*$. Without loss of generality, we assume $\upq^{T_1}$ satisfies $|\upq_{1:N}^{T_1}-\upv_{1:N}^*|\leq\frac{1}{4}\upv_{1:N}^*$ and $\boldsymbol{0}_{N+1:M}\leq\upq_{N+1:M}^{T_1}\leq\frac{3}{2}\upv_{N+1:M}^*$. Let $\hat{\tau}$ be the earliest time index satisfying $\calG^c(\tilde{\upv}^{\hat{\tau}})$, i.e.,
    \begin{align}
        \hat{\tau}=\inf\left\{t:\exists j\in[1:N], \text{ s.t. }\left|\tilde{\upv}_j^t-\upv_j^*\right|>\frac{1}{2}\upv_j^*\text{ or }\exists j\in[N+1:M], \text{ s.t. }\tilde{\upv}_j^t>2\upv_j^*\right\},\notag
    \end{align}
    For each coordinate $j\in[1:N]$, let $\hat{\tau}_{[1:N],j}^u$ and $\hat{\tau}_{[1:N],j}^l$ be the earliest time index satisfying $\widetilde{\upv}_j^{\hat{\tau}_{[1:N],j}^u}>\frac{3}{2}\upv_j^*$ and $\widetilde{\upv}_j^{\hat{\tau}_{[N+1:M],j}^l}<\frac{1}{2}\upv_j^*$, respectively, i.e.,
    $$
    \hat{\tau}_{[1:N],j}^u=\inf\left\{t: \widetilde{\upv}_j^t>\frac{3}{2}\upv_j^*\right\},\quad \hat{\tau}_{[1:N],j}^l=\inf\left\{t: \widetilde{\upv}_j^t<\frac{1}{2}\upv_j^*\right\}.
    $$
    For each coordinate $j\in[N+1:M]$, let $\hat{\tau}_{[N+1:M],j}$ be the earliest time index satisfying $\widetilde{\upv}_j^{\hat{\tau}_{[N+1:M],j}}>2\upv_j^*$, i.e.,
    $$
        \hat{\tau}_{[N+1:M],j}=\inf\left\{t: \widetilde{\upv}_j^t>2\upv_j^*\right\}.
    $$
    Once the stopping time $\hat{\tau}=t_2$ occurs for some $t_2\in[1:T_2]$, the coupling process satisfies $\tilde{\upv}^t=\tilde{\upv}^{t_2}$ for all $t>t_2$.
    
    Suppose there exists $j\in[1:N]$ such that $\hat{\tau}_{[1:N],j}^u=t_2$. Given stopping time $\hat{\tau}_{[1:N],j}^u=t_2$, the event $\calG(\tilde{\upv}^t)$ holds for all $t\in[0:t_2-1]$. Similarly, $\tilde{\upv}_j^t$ must sequentially enter and exit the threshold interval $[\upv_j^*,\frac{3}{2}\upv_j^*]$ before exceeding $\frac{3}{2}\upv_j^*$. We aim to estimate following probability for coordinates $j\in[1:N]$ and time pairs $t_1<t_2\in[0:T_2]$:
    % Moreover, for any fixed $t_0\in[0:\tau_u-1]$, we consider the event $\calB_{t_0}^{\tau_u}(j)=\{\widetilde{\upv}_j^{t_0}\leq\frac{5}{4}\upv_j^*\bigwedge\widetilde{\upv}_j^{t_0:\tau_u-1}\in[\frac{1}{2}\upv_j^*,\frac{3}{2}\upv_j^*]\}$. If $t\in[t_0:\tau_u-1]$ and $\calA(\widetilde{\upv}^t)$ holds, we obtain
    \begin{align}
        \bbP\left(\calB_{t_1}^{\hat{\tau}_{[1:N],j}^u=t_2}(j)=\left\{\widetilde{\upv}_j^{t_1}\leq\frac{5}{4}\upv_j^*\bigwedge\widetilde{\upv}_j^{t_1:t_2-1}\in\left[\upv_j^*,\frac{3}{2}\upv_j^*\right]\right\}\right).\notag
    \end{align}
    For any $t\in[t_1:t_2-1]$, we have
    \begin{equation}\label{mar-concen-4}
        \begin{split}
		\bbE\left[\widetilde{\upv}_j^{t+1}-\upv_j^*\mid\calF^t\right]=&\bbE_{\upx_{1:M}^{t+1},\xi^{t+1},\zeta_{M+1:\infty}^{t+1}}\left[\widetilde{\upv}_j^t-\upv_j^*-\eta\left(\left((\widetilde{\upv}_j^t)^2-(\upv_j^*)^2\right)\hat{\upx}_j^{t+1}+\hat{\upz}_j^{t+1}(\widetilde{\upv}^t)\right.\right.
        \\
        &\, \, \, \, \, \, \, \, \, \, \, \, \, \, \, \, \, \, \, \, \, \, \, \, \, \, \, \, \, \, \, \, \, \, \, \, \, \, \, \, \, \, \, \, \, \left.\left.-\hat{\zeta}_{M+1:\infty}^{t+1}-\hat{\xi}^{t+1}\right)\hat{\mathbf{x}}_j^{t+1}\widetilde{\mathbf{v}}_j^{t+1}\right]
		\\
		\leq&\left(1-\frac{3\eta_t}{8}\lambda_j(\upv_j^*)^2\right)(\widetilde{\upv}_j^t-\upv_j^*).
        \end{split}
	\end{equation}
	Applying Lemma \ref{aux-1} to $(((\widetilde{\upv}_j^t)^2-(\upv_j^*)^2)\hat{\upx}_j^{t+1}+\hat{\upz}_j^{t+1}(\widetilde{\upv}^t)-\hat{\zeta}_{M+1:\infty}^{t+1}-\hat{\xi}^{t+1})\hat{\mathbf{x}}_j^{t+1}\widetilde{\mathbf{v}}_j^{t+1}$, we obtain
	\begin{align}
		\bbE\left[\exp\left\{\lambda\left(\tilde{\upv}_j^{t+1}-\bbE\left[\tilde{\upv}_j^{t+1}\mid\calF^t\right]\right)\right\}\mid\calF^t\right]\leq\exp\left\{\frac{\lambda^2\eta_t^2\lambda_j(\upv_j^*)^2\calO\left(\left[\sigma^2+\mathcal{M}^2(\upb)\right]\log^4(MT_2/\delta)\right)}{2}\right\},\notag
	\end{align}
	for any $\lambda\in\bbR$. Therefore, combining Lemma \ref{aux-2} with Eq.~\eqref{mar-concen-4}, we further establish the probability bound for event $\calB_{t_1}^{\hat{\tau}_{[1:N],j}^u=t_2}(j)$ for any time pair $t_1<t_2\in[0:T_2]$.
	\begin{align}\label{phase_II_in_truncation}
		\Pro\left\{\calB_{t_1}^{\hat{\tau}_{[1:N],j}^u=t_2}(j)\right\}\leq\exp\left\{-\frac{(\upv_{j}^*)^2}{V_j}\right\},
	\end{align}
	where $V_j$ has the form of
	\begin{align}
		V_j=\lambda_j(\upv_j^*)^2\calO\left([\sigma^2+\mathcal{M}^2(\upb)]\log^4(MT_2/\delta)\right)\sum_{t=0}^{T_2-1}\left(\prod_{i=t+1}^{T_2-1}(1-\frac{3\eta_{i}}{4}\lambda_j(\upv_j^*)^2)^{2}\right)(\eta_t)^2.\notag
	\end{align}
	By Lemma \ref{aux-3}, we have $V_j\leq\calO(\eta_0[\sigma^2+\mathcal{M}^2(\upb)]\log^4(MT_2/\delta))$. Therefore, using Eq.~\eqref{phase_II_in_truncation}, we can derive 
    \begin{align}\label{prob-1}
    \Pro\left\{\calB_{t_1}^{\hat{\tau}_{[1:N],j}^u=t_2}(j)\right\}\leq\exp\left\{-\frac{(\upv_j^*)^2}{\eta_0\calO\left([\sigma^2+\mathcal{M}^2(\upb)]\log^4(MT_2/\delta)\right)}\right\}.
    \end{align}
    
    Suppose there exists $j\in[1:N]$ such that $\hat{\tau}_{[1:N],j}^l=t_2$. Given stopping time $\hat{\tau}_{[1:N],j}^l=t_2$, the event $\calG(\tilde{\upv}^t)$ holds for all $t\in[0:t_2-1]$. Similarly, $\tilde{\upv}_j^t$ must sequentially enter and exit the threshold interval $[\frac{1}{2}\upv_j^*,\upv_j^*]$ before subceeding $\frac{1}{2}\upv_j^*$. We aim to estimate following probability for coordinates $j\in[1:N]$ and time pairs $t_1<t_2\in[1:T_2]$: 
    \begin{align}
        \bbP\left(\calC_{t_1}^{\hat{\tau}_{[1:N],j}^l=t_2}(j)=\left\{\widetilde{\upv}_j^{t_1}\geq\frac{3}{4}\upv_j^*\bigwedge\widetilde{\upv}_j^{t_1:t_2-1}\in\left[\frac{1}{2}\upv_j^*,\upv_j^*\right]\right\}\right).\notag
    \end{align}
    For any $t\in[t_1:t_2-1]$, we have
    \begin{align}
        \bbE\left[\upv_j^*-\widetilde{\upv}_j^{t+1}\mid\calF^t\right]\leq\left(1-\frac{3\eta_t}{8}\lambda_j(\upv_j^*)^2\right)(\upv_j^*-\widetilde{\upv}_j^t).\notag
    \end{align}
    Applying Lemmas \ref{aux-1}, \ref{aux-2}, and \ref{aux-3} sequentially yields the probability bound for event $\calC_{t_1}^{\hat{\tau}_{[1:N],j}^l=t_2}(j)$ for any time pair $t_1<t_2\in[0:T_2]$ as follows:
    \begin{align}\label{prob-2}
		\Pro\left\{\calC_{t_1}^{\hat{\tau}_{[1:N],j}^l=t_2}(j)\right\}\leq\exp\left\{-\frac{(\upv_j^*)^2}{V_j}\right\}\leq\exp\left\{-\frac{(\upv_j^*)^2}{\eta_0\calO\left([\sigma^2+\mathcal{M}^2(\upb)]\log^4(MT_2/\delta)\right)}\right\}.
	\end{align}
	
	% In addition, we consider the component of $\widetilde{\upv}^{T_2}$ on $\bar{\calN}$ and define $\widehat{\tau}_u=\inf\{t\mid\widetilde{\upv}_j^t> 2\upv_{j}^*\}$ for any fixed index $j\in\bar{\calN}$. 
    Suppose there exists $j\in[N+1:M]$ such that $\hat{\tau}_{[N+1:M],j}=t_2$. Given stopping time $\hat{\tau}_{[N+1:M],j}=t_2$, the event $\calG(\tilde{\upv}^t)$ holds for all $t\in[0:t_2-1]$. Similarly, $\tilde{\upv}_j^t$ must sequentially enter and exit the threshold interval $[\upv_j^*,2\upv_j^*]$ before exceeding $2\upv_j^*$. We aim to estimate following probability for coordinates $j\in[N+1:M]$ and time pairs $t_1<t_2\in[0:T_2]$:
    \begin{align}
        \bbP\left(\calD_{t_1}^{\hat{\tau}_{[N+1:M],j}=t_2}(j)=\left\{\widetilde{\upv}_j^{t_1}\leq\frac{3}{2}\upv_j^*\bigwedge\widetilde{\upv}_j^{t_1:t_2-1}\in[\upv_j^*,2\upv_j^*]\right\}\right).\notag
    \end{align}
    For any $t\in[t_1:t_2-1]$, we have
	\begin{align}\label{mar-concen-5}
		\bbE\left[\widetilde{\upv}_j^{t+1}-\upv_j^*\mid\calF^t\right]\leq\widetilde{\upv}_j^{t}-\upv_j^*.
	\end{align}
	Applying Lemma \ref{aux-1} to $(((\widetilde{\upv}_j^t)^2-(\upv_j^*)^2)\hat{\upx}_j^{t+1}+\hat{\upz}_j^{t+1}(\widetilde{\upv}^t)-\hat{\zeta}_{M+1:\infty}^{t+1}-\hat{\xi}^{t+1})\hat{\mathbf{x}}_j^{t+1}\widetilde{\mathbf{v}}_j^{t+1}$, we obtain 
    \begin{align}
        \bbE\left[\exp\left\{\lambda\left(\tilde{\upv}_j^{t+1}-\bbE\left[\tilde{\upv}_j^{t+1}\mid\calF^t\right]\right)\right\}\mid\calF^t\right]\leq\exp\left\{\frac{\lambda^2\eta_t^2\lambda_j(\upv_j^*)^2\calO\left(\left[\sigma^2+\mathcal{M}^2(\upb)\right]\log^4(MT_2/\delta)\right)}{2}\right\},\notag
    \end{align}
    for any $\lambda\in\bbR$.
    % $\Var(j,t+1\mid t)\leq\frac{9(\eta_t)^2}{4}\lambda_j(\upv_j^*)^2\left[\sigma_{\xi}^2+\mathcal{M}^2(\upb)\right]$ 
    Therefore, combining Lemma \ref{aux-2} with Eq.~\eqref{mar-concen-5}, we further establish the probability bound for the event $\calD_{t_1}^{\hat{\tau}_{[N+1:M],j}=t_2}(j)$ for any time pair $t_1<t_2\in[0:T_2]$.
	\begin{align}\label{prob-3}
		\Pro\left\{\calD_{t_1}^{\hat{\tau}_{[N+1:M],j}=t_2}(j)\right\}\leq\exp\left\{-\frac{(\upv_j^*)^2}{V_j}\right\}\overset{\text{(a)}}{\leq}\exp\left\{-\frac{\log^{-4}(MT_2/\delta)}{T_2\eta_0^2\lambda_j\calO\left(\left[\sigma^2+\mathcal{M}^2(\upb)\right]\right)}\right\},
	\end{align}
	where (a) is derived from $V_j\leq T_2\eta_0^2\lambda_j\calO\left(\left[\sigma^2+\mathcal{M}^2(\upb)\right]\log^4(MT_2/\delta)\right)$.
	
	Observing that $\calG^c(\widetilde{\upv}^{T_2})$ indicates that one of the following: 
    \begin{enumerate}
        \item For some coordinates $j\in[1:N]$ and time pairs $t_1<t_2\in[0:T_2]$, either $\calB_{t_1}^{\hat{\tau}_{[1:N],j}^u=t_2}(j)$ or $\calC_{t_1}^{\hat{\tau}_{[1:N],j}^l=t_2}(j)$ occurs,
        \item For some coordinates $j\in[1:N]$ and time pairs $t_1<t_2\in[0:T_2]$, $\calD_{t_1}^{\hat{\tau}_{[N+1:M],j}=t_2}(j)$ occurs.
    \end{enumerate}
    Therefore, we derive the following probability bound of event $\calG^c(\widetilde{\upv}^{T_2})$:
	\begin{align}
		\Pro\{\calG^c(\widetilde{\upv}^{T_2})\}\leq&\sum_{t_1<t_2}\left[\sum_{j\in[1:N]}\left(\Pro\left\{\calB_{t_1}^{\hat{\tau}_{[1:N],j}^u=t_2}(j)\right\}+\Pro\left\{\calC_{t_1}^{\hat{\tau}_{[1:N],j}^l=t_2}(j)\right\}\right)\right.\notag
		\\
		&\, \, \, \, \, \, \, \, \, \, \, \, \, \, \left.+\sum_{j\in[N+1:M]}\Pro\left\{\calD_{t_1}^{\hat{\tau}_{[N+1:M],j}=t_2}(j)\right\}\right]
		\notag
		\\
		\leq&2T_2^2N\exp\left\{-\frac{\min_{j\in\calN}(\upv_j^*)^2}{\eta_0\calO\left([\sigma^2+\mathcal{M}^2(\upb)]\log^4(MT_2)\right)}\right\}
		\notag
		\\	
		&+T_2^2(\max\{M,N\}-N)\exp\left\{-\frac{\log^{-4}(MT_2/\delta)}{T_2\eta_0^2\max_{j\in\bar{\calN}}\lambda_j\calO\left(\left[\sigma^2+\mathcal{M}^2(\upb)\right]\right)}\right\}\notag
		\\
		\leq&\delta/2,\notag
	\end{align}
	using the setting of $\eta_0$. According to the construction of the coupling process $\{\tilde{\upv}^t\}_{t=0}^{T_2}$, we have that $\bigcap_{t=T_1}^{T_1+T_2}\calG(\upq^t)$ holds with probability at least $1-\delta/2$. By Proposition \ref{p1}, the proof is completed. 
\end{proof}

% Recalling the definition of auxiliary function $\psi$, if $\upv_{1:N}^{T_1+t+1}\in[\frac{1}{2}\upv_{1:N}^*,\frac{3}{2}\upv_{1:N}^*]$ and $\upv_{N+1:M}^{T_1+t+1}\in[\mathbf{0},2\upv_{N+1:M}^*]$ for any $t\in[0:T_2-1]$, we notice
Given the auxiliary function $\psi$, when the following bounds hold for all $t\in[0:T_2-1]$:
\begin{enumerate}
    \item For any $j\in[1:N]$, $\upv_{j}^{T_1+t+1}\in[\frac{1}{2}\upv_{j}^*,\frac{3}{2}\upv_{j}^*]$,
    \item For any $j\in[N+1:M]$, $\upv_{j}^{T_1+t+1}\in[0,2\upv_{j}^*]$,
\end{enumerate}
we observe that $\upw^{t+1}$ follows the update rule:
\begin{align}\label{iteration}
	\upw^{t+1}-\upv_{1:M}^*=\upw^t-\upv_{1:M}^*-\eta_t\upH_{\upw}^t\left(\upw^t-\upv_{1:M}^*\right)+\eta_t\upR_{\upw}^t\Pi_M\upx^t.
\end{align}
If the above bounds are violated, we enforce $\upw^{t+1}=\upv_{1:M}^*$. Consequently, we derive the recurrence process:
\begin{align}
\bbE\left[\left\|\upw^{t+1}-\upv_{1:M}^*\right\|^2\right]\leq\bbE\left[\left\|\upw^t-\upv_{1:M}^*-\eta_t\upH_{\upw}^t\left(\upw^t-\upv_{1:M}^*\right)+\eta_t\upR_{\upw}^t\Pi_M\upx^t\right\|^2\mathds{1}_{\upw^t=\upv^{T_1+t}}\right]\notag.
\end{align}
Moreover, we can obtain
\begin{align}
	&\bbE\left[\left(\upw^{t+1}-\upv_{1:M}^*\right)^{\otimes2}\right]\preceq\bbE\left[\left(\upw^t-\upv_{1:M}^*-\eta_t\upH_{\upw}^t\left(\upw^t-\upv_{1:M}^*\right)+\eta_t\upR_{\upw}^t\Pi_M\upx^t\right)^{\otimes2}\mathds{1}_{\upw^t=\upv^{T_1+t}}\right].\notag
\end{align}
According to the dynamics of $\upw^{t}-\upv_{1:M}^*$ discussed previously, we define $\widehat{\upw}^t:=\upw^t-\upv_{1:M}^*$. The iterative update of $\widehat{\upw}^t$ can be decomposed into two random processes,
\begin{align}
	\widehat{\upw}^{t}=\mathds{1}_{\upw^t=\upv^{T_1+t}}\cdot\widehat{\upw}_{\bi}^t+\mathds{1}_{\upw^t=\upv^{T_1+t}}\cdot\widehat{\upw}_{\var}^t,\quad \forall t\in[0:T_2],
\end{align}
where $\{\widehat{\upw}_{\var}^t\}_{t=1}^{T_2}$ is recursively defined by
\begin{align}
	\begin{cases}
		\widehat{\upw}_{\var}^{t+1}=\left(\upI-\eta_t\upH_{\upw}^t\right)\widehat{\upw}_{\var}^t+\eta_t\upR_{\upw}^t\Pi_M\upx^t,  & \text{ if }\upw^t=\upv^{T_1+t},
		\\\widehat{\upw}_{\var}^{t+1}=\mathbf{0}, & \text{ otherwise },
	\end{cases}\notag
\end{align}
for any $t\in[0:T_2-1]$ with $\widehat{\upw}_{\var}^0=\textbf{0}$ and $\{\widehat{\upw}_{\bi}^t\}_{t=1}^{T_2}$ is recursively defined by
\begin{align}
	\begin{cases}
		\widehat{\upw}_{\bi}^{t+1}=\left(\upI-\eta_t\upH_{\upw}^t\right)\widehat{\upw}_{\bi}^t, & \text{ if }\upw^t=\upv^{T_1+t},
		\\
		\widehat{\upw}_{\bi}^{t+1}=\mathbf{0}, & \text{ otherwise },\notag
	\end{cases}
\end{align}
for any $t\in[0:T_2-1]$ with  $\widehat{\upw}_{\bi}^0=\upw^0-\upv_{1:M}^*$. We define the $t$-th step bias iterate $\upB^t=\bbE\left[\widehat{\upw}_{\bi}^t\otimes\widehat{\upw}_{\bi}^t\right]$ and $t$-th step variance iterate $\upV^t=\bbE\left[\widehat{\upw}_{\var}^t\otimes\widehat{\upw}_{\var}^t\right]$.
Therefore, we can derive the following relations for 
$\{\upB^t\}_{t=0}^{T_2}$ and $\{\upV^t\}_{t=0}^{T_2}$:
\begin{align}
	\begin{cases}\label{bias-and-variance}
        \upB^{t+1}&\preceq\bbE\left[\left(\calI-\eta_t\calG_{\upw}^t\right)\circ\left(\widehat{\upw}_{\bi}^t\otimes\widehat{\upw}_{\bi}^t\right)\right],
		\\
		\upV^{t+1}&\preceq\bbE\left[\left(\calI-\eta_t\calG_{\upw}^t\right)\circ\left(\widehat{\upw}_{\var}^t\otimes\widehat{\upw}_{\var}^t\right)\right]+\eta_t^2\upSigma_{\upw}^t,
	\end{cases}\quad \forall t\in[0:T_2-1],
\end{align}
with $\upB^0=\left(\upw^0-\upv_{1:M}^*\right)\left(\upw^0-\upv_{1:M}^*\right)^{\top}$ and $\upV^0=\mathbf{0}$, where $\upSigma_{\upw}^t=\sigma^2\upLambda\diag\{\upw^t\odot\upw^t\}$. Then, we can drive following estimation of last-iterate function value:
\begin{align}
	\bbE\left[\calR_M(\upw^{T_2})-\calR_M(\upv_{1:M}^*)\right]\leq\frac{1}{2}\llangle\upH,\bbE\left[\widehat{\upw}^{T_2}\otimes\widehat{\upw}^{T_2}\right]\rrangle\leq\llangle\upH,\upB^{T_2}\rrangle+\llangle\upH,\upV^{T_2}\rrangle,
\end{align}
where $\upH=\frac{25}{4}\upLambda\diag\{\widehat{\upb}\odot\widehat{\upb}\}$ and $\widehat{\upb}^{\top}=\left((\upv_{1:N}^*)^{\top},(\widehat{\upv}_{N+1:M}^*)^{\top}\right)$. From the definitions of $\upw^t$ and $\upH_{\upw}^t$, we observe that $\bbE[\upH_{\upw}^t]\preceq\upH$. We use $\widehat{\upH}$ to denote $\frac{1}{4}\upLambda\diag\{\overline{\upb}\odot\overline{\upb}\}$ where $\overline{\upb}^{\top}=\left((\upv_{1:N}^*)^{\top},\mathbf{0}^{\top}\right)$, and define $\widehat{\calG}:=\widehat{\upH}\otimes\upI+\upI\otimes\widehat{\upH}-\eta\widehat{\upH}\otimes\widehat{\upH}$. Combining Lemma \ref{high-probability-phase-II} with the results in section \ref{sec-variance} and \ref{sec-bias}, we obtain following estimation of $\calR_M(\upv^{T_2})-\calR_M(\upv_{1:M}^*)$:
\begin{theorem}\label{phase-II-main}
    Suppose Assumption \ref{ass-d} and Assumption \ref{ass-s} hold and let $T_1=\lceil(T_1+T_2-h)/\log(T_1+T_2-h)\rceil$.
    Under the following setting
    \begin{enumerate}
        \item There exists $N<M$ such that $\eta_0\leq\widetilde{\Theta}(\min\{((C+2)\tr(\upH))^{-1},\Barsigmin(N)\})$ and $T_1=\widetilde{\calO}(\frac{\sigma^2+\calM^2(\widehat{\upb})}{\eta_0\sigmin(N)})$,
        \item Let $N=M$, $\eta_0\leq\widetilde{\Theta}(\min\{((C+2)\tr(\upH))^{-1},\Barsigmin(M)\})$, and $T_1\geq\widetilde{\calO}(\frac{\sigma^2+\calM^2(\widehat{\upb})}{\eta_0\sigmin(M)})$,
    \end{enumerate}
    we have
    \begin{align}\label{phaseII-p1}
        \bbE\left[\calR_M(\upw^{T_2})-\calR_M(\upv_{1:M}^*)\right]\lesssim&\sigma^2\left(\frac{N_0'}{K}+\eta_0\sum_{i=N_0'+1}^{N_0}\lambda_i(\upv_i^*)^2\right)\notag
        \\
        &+\sigma^2\eta_0^2(h+K)\sum_{i=N_0+1}^M\lambda_i^2(\widehat{\upb}_i^*)^4\notag
        \\
        &+\llangle\frac{1}{\eta_0 K}\upI_{1:N_1}+\upH_{N_1+1:M},\left(\upI-\eta_0\widehat{\upH}\right)^{2h}\upB^0\rrangle\notag
        \\
        &+(C+2)\Gamma_K(\upH)\llangle\frac{1}{\eta_0h}\upI_{1:N_1'}+\upH_{N_1'+1:M},\upB^0\rrangle,
    \end{align}
    for arbitrary $N\geq N_0\geq N_0'\geq 0$ and $N\geq N_1\geq N_1'\geq 0$, where $\Gamma_K(\upH):=(\frac{625N_1'}{K}+\frac{25\eta_0h}{K}\tr(\upH_{N_1'+1:N_1})+\eta_0^2h\tr(\upH_{N_1+1:M}^2))$. Specially, we have 
    \begin{equation}\label{phaseII-p2}
        \begin{split}
        \calR_M(\upv^{T_1+T_2})-\calR_M(\upv_{1:M}^*)\lesssim&\frac{\sigma^2N}{K}+\sigma^2\eta_0^2(h+K)\sum_{i=N+1}^M\lambda_i^2(\widehat{\upb}_i^*)^4
        \\
        &+\llangle\frac{1}{\eta_0 K}\upI_{1:N}+\upH_{N+1:M},\left(\upI-\eta_0\widehat{\upH}\right)^{2h}\upB^0\rrangle
        \\
        &+(C+2)\left(\frac{N}{K}+\eta_0^2h\tr(\upH_{N+1:M}^2)\right)\llangle\frac{1}{\eta_0h}\upI_{1:N}+\upH_{N+1:M},\upB^0\rrangle,
        \end{split}
    \end{equation}
    with probability at least 0.95.
\end{theorem}
\begin{proof}
    Combining Theorem \ref{variance-upper-bound} with Theorem \ref{bias-upper-bound}, we derive Eq.~\eqref{phaseII-p1}. Based on Lemma \ref{high-probability-phase-II}, the equality $\upw^{T_2}=\upv^{T_1+T_2}$ holds with probability at least $1-\delta$. By setting $N_0'=N_0=N_1'=N_1=N$ in Eq.~\eqref{phaseII-p1} and applying Markov's inequality, we obtain Eq.~\eqref{phaseII-p2}.
\end{proof}

\subsubsection{Bound of Variance}\label{sec-variance}
Lemma \ref{primal-var-estimation} provides a uniform upper bound for $\upV^t$ over $t\in[0:T_2]$. 
% The proof of Lemma \ref{primal-var-estimation} draws on the relevant proof techniques from \citet{Belkin2019TwoMO,ge2019step,wu2022last}.
\begin{lemma}\label{primal-var-estimation}
    Suppose Assumption \ref{ass-d} holds. Under the setting of Theorem \ref{phase-II-main}, for any $t\in[0:T_2]$, we obtain
    \begin{align}
        \upV_{\diag}^{t}\precsim\eta_0\sigma^2\upI.
    \end{align}
\end{lemma}
\begin{proof}
    It can be observed that $\upSigma_{\upw}^t\preceq\sigma^2\bbE[\upH_{\upw}^t]\preceq\upH$, given that $\upv_{1:M}^*\geq\mathbf{0}$. The proof relies on induction. At $t=0$, it follows that $\upV_{\diag}^0=\mathbf{0}\precsim\eta_0\sigma^2\upI$. Assuming $\upV_{\diag}^{\tau}\precsim\eta_0\sigma^2\upI$ for any $\tau\leq t$, we proceed to estimate $\upV^{t+1}$ by combining Eq.~\eqref{bias-and-variance},
    \begin{align}
        \upV_{\diag}^{t+1}\preceq&\left(\bbE\left[\left(\calI-\eta_t\calG_{\upw}^t\right)\circ\left(\widehat{\upw}_{\var}^t\otimes\widehat{\upw}_{\var}^t\right)\right]\right)_{\diag}+\eta_t^2\upSigma_{\upw}^t\notag\\
        \preceq&\left(\calI-\eta_t\widehat{\upH}\otimes\upI-\eta_t\upI\otimes\widehat{\upH}\right)\circ\upV_{\diag}^{t}\notag
        \\
        &+\eta_t^2\left(\bbE\left[\calH_{\upw}^t\circ\left(\widehat{\upw}_{\var}^t\otimes\widehat{\upw}_{\var}^t\right)\right]\right)_{\diag}+\eta_t^2\sigma^2\upH\notag
        \\
        \overset{\text{(a)}}{\preceq}&\left(\upI-2\eta_t\widehat{\upH}\right)\upV_{\diag}^{t}+\calO\left(\eta_t^2 (C+2)\langle\upH,\upV_{\diag}^{t}\rangle\upH+\eta_t^2\sigma^2\upH\right)\notag
        \\
        \preceq&\left(\upI-2\eta_t\widehat{\upH}\right)\upV_{\diag}^{t}+\widetilde{\calO}\left(\eta_t^2\eta_0\sigma^2 (C+2)\tr(\upH)\upH+\eta_t^2\sigma^2\upH\right),\notag
    \end{align}
    where (a) is derived from applying Lemma \ref{aux-6} with $\upA=\diag\{\upv_{1:M}^*+\upw^t\}$ and $\upB=\widehat{\upw}_{\var}^t\otimes\widehat{\upw}_{\var}^t$. For $i\in[1:N]$, we have
    \begin{align}\label{eq-var-1}
        \left(\upV_{\diag}^{t+1}\right)_{i,i}\leq\left(1-2\eta_t\widehat{\upH}_{i,i}\right)\left(\upV_{\diag}^{t}\right)_{i,i}+\widetilde{\calO}\left(\eta_t^2\sigma^2\widehat{\upH}_{i,i}\right).
    \end{align}
    The recursive expression given by Eq.~\eqref{eq-var-1} implies that $(\upV_{\diag}^{t+1})_{i,i}\lesssim\eta_0\sigma^2$ for any $i\in[1:N]$, using Lemma \ref{aux-3}. For $i\in[N+1:M]$, we obtain
    \begin{align}
        \left(\upV_{\diag}^{t+1}\right)_{i,i}\lesssim\sigma^2\widehat{\upH}_{i,i}\sum_{k=0}^t\eta_k^2\lesssim\eta_0\sigma^2.
    \end{align}
    % Since $\eta_0>\eta_t$ and $\bbE[\upH_{\upw}^t]\succeq\mathbf{0}$, we have $\upV^{t+1}\preceq\frac{\eta_0\sigma^2}{1-\eta_0R^2}\upI$. 
    Therefore, we complete the induction.
\end{proof}
\begin{theorem}\label{variance-upper-bound}
    Suppose Assumption \ref{ass-d} holds. Under the setting of Theorem \ref{phase-II-main}, we have
    \begin{align}
        \llangle\upH,\upV^{T_2}\rrangle\lesssim&\sigma^2\left(\frac{N_0'}{K}+\eta_0\sum_{i=N_0'+1}^{N_0}\lambda_i(\upv_i^*)^2\right)+\sigma^2\eta_0^2(h+K)\sum_{i=N_0+1}^M\lambda_i^2(\widehat{\upb}_i^*)^4,
    \end{align}
    for arbitrary $N\geq N_0\geq N_0'\geq0$.
\end{theorem}
\begin{proof}
    % By selecting $\upA=\diag\{\upw^t\}$ and $\upB=\diag^2\{\upw^t+\upv_{1:M}^*\}\diag^{-2}\{\upw^t\}$ in Lemma \ref{aux-6}, we derive the inequality $\bbE[\upH^t(\upH^t)^{\top}]\preceq (C+2)\tr(\upH)\bbE[\upH^t]$. 
    Applying Eq.~\eqref{bias-and-variance}, we obtain
    \begin{align}\label{express-V}
        \upV_{\diag}^{t+1}\preceq&\left(\calI-\eta_t\widehat{\calG}\right)\circ\upV_{\diag}^t+\eta_t^2\left(\calH_{\upw}^t\circ\left(\widehat{\upw}_{\var}^t\otimes\widehat{\upw}_{\var}^t\right)\right)_{\diag}+\eta_t^2\sigma^2\bbE[\upH_{\upw}^t]\notag
        \\
        \overset{\text{(a)}}{\preceq}&\left(\calI-\eta_t\widehat{\calG}\right)\circ\upV_{\diag}^t+\widetilde{\calO}\left(\eta_t^2\sigma^2\eta_0(C+2)\tr(\upH)\upH+\eta_t^2\sigma^2\upH\right)\notag
        \\
        =&\left(\calI-\eta_t\widehat{\calG}\right)\circ\upV_{\diag}^t+\widetilde{\calO}\left(\eta_t^2\sigma^2\upH\right),
    \end{align}
    where (a) is derived from Lemma \ref{primal-var-estimation}. Therefore, the recursive expression for $\upV^{T_2}$ can be directly derived by incorporating Eq.~\eqref{express-V}.
    \begin{align}\label{recur-variance}
        \upV_{\diag}^{T_2}\precsim\sigma^2\sum_{t=0}^{T_2}\eta_t^2\prod_{i=t+1}^{T_2}\left(\calI-\eta_i\widehat{\calG}\right)\circ\upH
        % \overset{\text(b)}{\preceq}&\frac{\sigma^2}{1-\eta_0 (C+2)\tr(\upH)}\sum_{t=0}^{T_2}\eta_t^2\prod_{i=t+1}^{T_2}\left(\upI-\eta_i\bbE[\upH_{\upw}^i]\right)\bbE[\upH_{\upw}^t]\notag
        % \\
        \overset{\text(b)}{\precsim}\sigma^2\underbrace{\sum_{t=0}^{T_2}\eta_t^2\prod_{i=t+1}^{T_2}\left(\upI-\eta_i\widehat{\upH}\right)\upH}_{\lai}.
    \end{align}
    (b) follows from the inequality $(1-\eta c_2)^2c_3\leq(1-\eta c_2)c_3$, which holds for any $\eta\leq c_2^{-1}$ given fixed constants $c_2,c_3>0$. 
    % Additionally, (c) is derived from the estimation $\widehat{\upH}\preceq\bbE[\upH^i]$, which holds for all $i\in[1:T_2]$. 
    According to the update rule for $\eta_t$ defined in Algorithm \ref{SGD}, we obtain
    \begin{align}\label{eq-variance-I}
        \lai=&\eta_0^2\sum_{i=1}^h\left(\upI-\eta_0\widehat{\upH}\right)^{h-i}\prod_{j=1}^{L}\left(\upI-\frac{\eta_0}{2^j}\widehat{\upH}\right)^K\upH\notag
        \\
        &+\sum_{l=1}^{L}\left(\frac{\eta_0}{2^l}\right)^2\sum_{i=1}^K\left(\upI-\frac{\eta_0}{2^l}\widehat{\upH}\right)^{K-i}\prod_{j=l+1}^{L}\left(\upI-\frac{\eta_0}{2^j}\widehat{\upH}\right)^K\upH\notag
        \\
        \preceq&4\left(\left(\frac{\eta_0}{2}\right)^2\sum_{i=1}^{h+K}\left(\upI-\frac{\eta_0}{2}\widehat{\upH}\right)^{h+K-i}\prod_{j=1}^{L-1}\left(\upI-\frac{\eta_0}{2^{1+j}}\widehat{\upH}\right)^K\upH\right.\notag
        \\
        &\, \, \, \, \, \, \, \, +\left.\sum_{l=1}^{L-1}\left(\frac{\eta_0}{2^{1+l}}\right)^2\sum_{i=1}^K\left(\upI-\frac{\eta_0}{2^{1+l}}\widehat{\upH}\right)^{K-i}\prod_{j=l+1}^{L-1}\left(\upI-\frac{\eta_0}{2^{1+j}}\widehat{\upH}\right)^K\upH\right)\notag
        \\
        \preceq&100\left(\frac{\eta_0}{2}\left(\upI-\left(\upI-\frac{\eta_0}{2}\widehat{\upH}_{1:N}\right)^{s+K}\right)\prod_{j=1}^{L-1}\left(\upI-\frac{\eta_0}{2^{1+j}}\widehat{\upH}_{1:N}\right)^K\right.\notag
        \\
        &\, \, \, \, \, \, \, \, \, \, \, \, \, \, +\left.\sum_{l=1}^{L-1}\frac{\eta_0}{2^{1+l}}\left(\upI-\left(\upI-\frac{\eta_0}{2^{1+l}}\widehat{\upH}_{1:N}\right)^K\right)\prod_{j=l+1}^{L-1}\left(\upI-\frac{\eta_0}{2^{1+j}}\widehat{\upH}_{1:N}\right)^K\right)\notag
        \\
        &+2\eta_0^2(h+K)\upH_{N+1:M}.
    \end{align}
    Therefore, we define the following scalar function
    \begin{align}
        f(x):=x\left(1-(1-x)^{h+K}\right)\prod_{j=1}^{L-1}\left(1-\frac{x}{2^j}\right)^K+\sum_{l=1}^{L-1}\frac{x}{2^l}\left(1-\left(1-\frac{x}{2^l}\right)^K\right)\prod_{j=l+1}^{L-1}\left(1-\frac{x}{2^j}\right)^K,\notag
    \end{align}
    as similar as that in [Lemma C.2, \citet{wu2022last}]. Moreover, the following inequality can be directly derived
    \begin{align}\label{aux-scalar-func}
        f\left(\frac{\eta_0}{2}\widehat{\upH}_{1:N}\right)\preceq\frac{8}{K}\upI_{1:N_0'}+\eta_0\widehat{\upH}_{N_0'+1:N_0}+\frac{\eta_0^2}{2}(h+K)\widehat{\upH}_{N_0+1:N}^2,
    \end{align}
    for arbitrary $N\geq N_0\geq N_0'\geq0$ by [Lemma C.3, \citet{wu2022last}]. Applying Eq.~\eqref{aux-scalar-func} to Eq.~\eqref{eq-variance-I} and combining Eq.~\eqref{recur-variance}, we obtain
    \begin{align}
        \upV_{\diag}^{T_2}\precsim&\sigma^2\left(\frac{1}{K}\widehat{\upH}_{1:N_0'}^{-1}+\eta_0\upI_{N_0'+1:N_0}+\eta_0^2(h+K)\widehat{\upH}_{N_0+1:N}+\eta_0^2(h+K)\upH_{N+1:M}\right).
    \end{align}
    Consequently, we have
    \begin{align}
        \llangle\upH,\upV^{T_2}\rrangle\lesssim&\sigma^2\left(\frac{N_0'}{K}+\eta_0\tr\left(\widehat{\upH}_{N_0'+1:N_0}\right)+\eta_0^2(h+K)\tr\left(\widehat{\upH}_{N_0+1:N}^2\right)\right)\notag
        \\
        &+\sigma^2\eta_0^2(h+K)\tr\left(\upH_{N+1:M}^2\right)\notag
        \\
        \lesssim&\sigma^2\left(\frac{N_0'}{K}+\eta_0\sum_{i=N_0'+1}^{N_0}\lambda_i(\upv_i^*)^2\right)+\sigma^2\eta_0^2(h+K)\sum_{i=N_0+1}^M\lambda_i^2(\widehat{\upb}_i^*)^4.
    \end{align}
\end{proof}

\subsubsection{Bound of Bias}\label{sec-bias}
This section begins with an analysis of the bias error during a single period of Algorithm \ref{SGD}, where the bias iterates are updated using a constant step size $\eta_t\equiv\eta$ over $\hat{T}$ steps. Based on Eq.~\eqref{bias-and-variance}, the bias iterates are updated according to the following rule:
\begin{align}\label{recur-bias}
    \upB^{t+1}\preceq\bbE\left[\left(\calI-\eta\calG_{\upw}^t\right)\circ\left(\widehat{\upw}_{\bi}^t\otimes\widehat{\upw}_{\bi}^t\right)\right],\quad \forall t\in[0:\hat{T}-1].
\end{align}
Combining Eq.~\eqref{recur-bias}, we have
\begin{align}\label{period-bias}
    \upB_{\diag}^{t+1}\preceq&\left(\calI-\eta\widehat{\calG}\right)\circ\upB_{\diag}^t+\eta^2\bbE\left(\left[\calH_{\upw}^t\circ\upB^t\right]\right)_{\diag}\notag
    \\
    \preceq&\prod_{i=0}^t\left(\calI-\eta\widehat{\calG}\right)\circ\upB_{\diag}^0+\eta^2\sum_{i=0}^{t}\prod_{j=i+1}^{t}\left(\calI-\eta\widehat{\calG}\right)\circ\bbE\left(\left[\calH_{\upw}^t\circ\upB^t\right]\right)_{\diag}\notag
    \\
    \overset{\text{(a)}}{\preceq}&\prod_{i=0}^t\left(\calI-\eta\widehat{\calG}\right)\circ\upB_{\diag}^0+(C+2)\eta^2\sum_{i=0}^{t}\prod_{j=i+1}^{t}\left(\calI-\eta\widehat{\calG}\right)\circ\upH\llangle\upH,\upB^i\rrangle.
\end{align}
where (a) is derived from Lemma \ref{aux-6} by selecting $\upA=\frac{5}{2}\diag\{\widehat{\upb}\}$ and $\upB=\upB^i$. According to Eq.~\eqref{period-bias}, it can be observed that
\begin{align}\label{diag-bias}
    \upB_{\diag}^{t+1}\preceq\left(\calI-\eta\widehat{\calG}\right)^{t+1}\circ\upB_{\diag}^0+(C+2)\eta^2\sum_{i=0}^{t}\left(\upI-\eta\widehat{\upH}\right)^{2(t-i)}\upH\llangle\upH,\upB^i\rrangle.
\end{align}
We utilize the following lemma to estimate $\llangle\upH,\upB^{\hat{T}}\rrangle$ under bias iteration defined in Eq.~\eqref{recur-bias}.
\begin{lemma}\label{period-bias-lemma}
    Suppose Assumption \ref{ass-d} and Assumption \ref{ass-s} hold, and $\upB^t$ is recursively defined by Eq.~\eqref{recur-bias}. Under the setting of Theorem \ref{phase-II-main}, letting $1\leq\hat{T}\leq T$ and $\eta\leq\eta_0$, we have
    \begin{align}
        \llangle\upH,\upB^{\hat{T}}\rrangle\leq\frac{2}{1-\widetilde{\calO}(C+2)\eta\tr(\upH)}\llangle\frac{25}{\eta \hat{T}}\upI_{1:N_0}+\upH_{N_0+1:M},\upB^0\rrangle,
    \end{align}
    where $N_0\in[0:N]$ is an arbitrary integer.
\end{lemma}
\begin{proof}
    By Lemma \ref{aux-5}, we can derive $\eta(\upI-\eta\widehat{\upH})^{2t}\upH\preceq\frac{25}{t+1}\upI$. Applying this to Eq.~\eqref{diag-bias}, we obtain
    \begin{align}\label{bias-eq-1}
        \upB_{\diag}^{t+1}\preceq\left(\calI-\eta\widehat{\calG}\right)^{t+1}\circ\upB_{\diag}^0+25(C+2)\eta\sum_{i=0}^t\frac{\llangle\upH,\upB^i\rrangle}{t+1-i}\cdot\upI,
    \end{align}
    for any $t\in[0:\hat{T}-1]$. Therefore, utilizing Lemma \ref{aux-7}, we have
    \begin{align}\label{equation-sum}
        \sum_{i=0}^{t}\frac{\llangle\upH,\upB^i\rrangle}{t+1-i}\leq\llangle\sum_{i=0}^t\frac{(\upI-\eta\widehat{\upH})^{2i}\upH}{t+1-i},\upB^0\rrangle+\widetilde{\calO}(C+2)\eta\tr(\upH)\sum_{i=0}^t\frac{\llangle\upH,\upB^i\rrangle}{t+1-i},
    \end{align}
    for any $t\in[1:\hat{T}]$. Eq.~\eqref{equation-sum} implicates that 
    \begin{align}\label{bias-eq-2}
        \sum_{t=0}^{\hat{T}-1}\frac{\llangle\upH,\upB^t\rrangle}{\hat{T}-t}\leq\frac{1}{1-\widetilde{\calO}(C+2)\eta\tr(\upH)}\llangle\sum_{t=0}^{\hat{T}-1}\frac{(\upI-\eta\widehat{\upH})^{2t}\upH}{\hat{T}-t},\upB^0\rrangle,
        %分母为1-2\calO(C+2)\log(T)^3\log(\delta^{-1})\eta\tr(\upH)
    \end{align}
    since $\widetilde{\calO}\eta(C+2)\tr(\upH)<1$. Combining Eq.~\eqref{bias-eq-1} with Eq.~\eqref{bias-eq-2}, we obtain
    \begin{align}\label{bias-eq-3}
        \llangle\upH,\upB^{\hat{T}}\rrangle\leq&\llangle(\upI-\eta\widehat{\upH})^{2\hat{T}}\upH,\upB^0\rrangle+\frac{{\calO}(C+2)\eta\tr(\upH)}{1-\widetilde{\calO}(C+2)\eta\tr(\upH)}\llangle\sum_{t=0}^{\hat{T}-1}\frac{(\upI-\eta\widehat{\upH})^{2t}\upH}{\hat{T}-t},\upB^0\rrangle\notag
        \\
        \overset{\text{(a)}}{\leq}&\llangle(\upI-\eta\widehat{\upH})^{2\hat{T}}\upH,\upB^0\rrangle\notag
        \\
        &+\frac{{\calO}(C+2)\eta\tr(\upH)}{1-\widetilde{\calO}(C+2)\eta\tr(\upH)}\llangle\frac{\upI_{1:N}-(\upI_{1:N}-\eta\widehat{\upH}_{1:N})^{\hat{T}}}{\eta \hat{T}}+(\upI_{1:N}-\eta\widehat{\upH}_{1:N})^{\hat{T}}\widehat{\upH}_{1:N},\upB^0\rrangle\notag
        \\
        &+\frac{{\calO}(C+2)\eta\tr(\upH)}{1-\widetilde{\calO}(C+2)\eta\tr(\upH)}\llangle\upH_{N+1:M},\upB^0\rrangle\notag
        \\
        \overset{\text(b)}{\leq}&\frac{2}{1-\widetilde{\calO}(C+2)\eta\tr(\upH)}\llangle\frac{25}{\eta T}\upI_{1:N_0}+\upH_{N_0+1:M},\upB^0\rrangle,
    \end{align}
    where $N_0\in[0:N]$ is an arbitrary integer,  (a) follows from the trick established in [Lemma C.4, \citet{wu2022last}], and (b) is derived from the invariant scaling relationship between $\widehat{\upH}_{1:N}$ and $\upH_{1:N}$. 
\end{proof}

\begin{lemma}\label{bias-diag}
    Suppose Assumption \ref{ass-d} and Assumption \ref{ass-s} hold. Under the setting of Theorem \ref{phase-II-main}, letting $2\leq\hat{T}\leq T$ and $\eta\leq\eta_0$, we have
    \begin{align}
        \upB_{\diag}^{\hat{T}}\preceq\left(\upI-\eta\widehat{\upH}\right)^{\hat{T}}\upB_{\diag}^0\left(\upI-\eta\widehat{\upH}\right)^{\hat{T}}+\frac{\widetilde{\calO}(C+2)\eta^2\hat{T}}{1-\widetilde{\calO}(C+2)\eta\tr(\upH)}\llangle\widetilde{\upH}^{\hat{T}},\upB^0\rrangle\overline{\upH}^{\hat{T}},
    \end{align}
    where $\widetilde{\upH}^{t}:=\frac{25}{\eta t}\upI_{1:N_0}+\upH_{N_0+1:M}$, and $\overline{\upH}^{t}:=\frac{25}{\eta t}\upI_{1:N_0'}+\upH_{N_0'+1:M}$ for any $t\geq1$, and $N_0,N_0'\in[0:N]$ could be arbitrary integer.
\end{lemma}
\begin{proof}
    Applying Lemma \ref{period-bias-lemma} into Eq.~\eqref{diag-bias}, we obtain
    \begin{align}\label{bias-lemma-1-main}
        \upB_{\diag}^{\hat{T}}\preceq&\left(\calI-\eta\widehat{\calG}\right)^{\hat{T}}\circ\upB_{\diag}^0+(C+2)\eta^2\left(\upI-\eta\widehat{\upH}\right)^{2(\hat{T}-1)}\upH\llangle\upH,\upB^0\rrangle\notag
        \\
        &+(C+2)\eta^2\sum_{t=1}^{\hat{T}-1}\left(\upI-\eta\widehat{\upH}\right)^{2(\hat{T}-1-t)}\upH\llangle\upH,\upB^t\rrangle\notag
        \\
        \preceq&\left(\calI-\eta\widehat{\calG}\right)^{\hat{T}}\circ\upB_{\diag}^0+(C+2)\eta^2\underbrace{\left(\upI-\eta\widehat{\upH}\right)^{2(\hat{T}-1)}\upH\llangle\upH,\upB^0\rrangle}_{\calcolI}\notag
        \\
        &+\frac{2(C+2)\eta^2}{1-2\widetilde{O}(C+2)\eta\tr(\upH)}\underbrace{\sum_{t=1}^{\hat{T}-1}\left(\upI-\eta\widehat{\upH}\right)^{2(\hat{T}-1-t)}\upH\llangle\widetilde{\upH}^t,\upB^0\rrangle}_{\calcolII},
    \end{align}
    We then provide a bound of term $\calcolII$ as follows:
    \begin{align}
        \calcolII=&\left(\sum_{t=1}^{\hat{T}-1}\llangle\widetilde{\upH}^t,\upB^0\rrangle\right)\upH_{N+1:M}+25\sum_{t=1}^{\hat{T}-1}\left(\upI_{1:N}-\eta\widehat{\upH}_{1:N}\right)^{2(\hat{T}-1-t)}\widehat{\upH}_{1:N}\llangle\widetilde{\upH}^t,\upB^0\rrangle\notag
        \\
        \preceq&\hat{T}\log(\hat{T})\llangle\widetilde{\upH}^{\hat{T}},\upB^0\rrangle\upH_{N+1:M}+25\left(\sum_{t=1}^{\hat{T}/2-1}\left(\upI_{1:N}-\eta\widehat{\upH}_{1:N}\right)^{\hat{T}}\widehat{\upH}_{1:N}\llangle\widetilde{\upH}^t,\upB^0\rrangle\right.\notag
        \\
        &+\left.\sum_{t=\hat{T}/2}^{\hat{T}-1}\left(\upI_{1:N}-\eta\widehat{\upH}_{1:N}\right)^{\hat{T}-1-t}\widehat{\upH}_{1:N}\llangle\widetilde{\upH}^{\hat{T}/2},\upB^0\rrangle\right)\notag
        \\
        =&\hat{T}\log(\hat{T})\llangle\widetilde{\upH}^{\hat{T}},\upB^0\rrangle\upH_{N+1:M}+25\left(\left(\upI_{1:N}-\eta\widehat{\upH}_{1:N}\right)^{\hat{T}}\widehat{\upH}_{1:N}\llangle\sum_{t=1}^{\hat{T}/2-1}\widetilde{\upH}^t,\upB^0\rrangle\right.\notag
        \\
        &+\left.\frac{\upI_{1:N}-\left(\upI_{1:N}-\eta\widehat{\upH}_{1:N}\right)^{\hat{T}/2}}{\eta}\llangle\widetilde{\upH}^{\hat{T}/2},\upB^0\rrangle\right)\notag
        \\
        \preceq&\hat{T}\log(\hat{T})\llangle\widetilde{\upH}^{\hat{T}},\upB^0\rrangle\upH_{N+1:M}+25\left(\hat{T}\log(\hat{T})\left(\upI_{1:N}-\eta\widehat{\upH}_{1:N}\right)^{\hat{T}}\widehat{\upH}_{1:N}\llangle\widetilde{\upH}^{\hat{T}},\upB^0\rrangle\right.\notag
        \\
        &+2\left.\frac{\upI_{1:N}-\left(\upI_{1:N}-\eta\widehat{\upH}_{1:N}\right)^{\hat{T}/2}}{\eta}\llangle\widetilde{\upH}^{\hat{T}},\upB^0\rrangle\right)\notag
        \\
        \overset{\text{(a)}}{\preceq}& \hat{T}\log(\hat{T})\llangle\widetilde{\upH}^{\hat{T}},\upB^0\rrangle\overline{\upH}^{\hat{T}},
    \end{align}
    where (a) follows from adapting the methodology from Eq.~\eqref{bias-eq-3}. We then proceed to establish bounds on $\calcolI$. It's worth to notice that
    \begin{align}\label{sub-1}
        \left(\upI-\eta\widehat{\upH}\right)^{2(\hat{T}-1)}\upH\preceq\frac{25}{2\eta(\hat{T}-1)}\upI_{1:N_0'}+25\widehat{\upH}_{N_0'+1:N}+\upH_{N+1:M}\preceq\overline{\upH}^{\hat{T}}.
    \end{align}
    Applying Eq.~\eqref{sub-1} into the definition of $\calcolI$, we obtain
    \begin{align}
        \calcolI\preceq\overline{\upH}^{\hat{T}}\llangle\upH,\upB^0\rrangle\preceq \hat{T}\overline{\upH}^{\hat{T}}\llangle\widetilde{\upH}^{\hat{T}},\upB^0\rrangle,
    \end{align}
    where the last inequality is derived from the condition $\eta<1/(25\tr(\upH))$, which ensures $\lambda_i(\upH)<1/\eta$ holds for all $i\in[1:N_0]$. Bringing the estimation of $\calcolI$ and $\calcolII$ into Eq.~\eqref{bias-lemma-1-main} yields
    \begin{align}
        \upB_{\diag}^{\hat{T}}\preceq&\left(\calI-\eta\widehat{\calG}\right)^{\hat{T}}\circ\upB_{\diag}^0+(C+2)\eta^2\hat{T}\widetilde{\upH}^{\hat{T}}\llangle\widetilde{\upH}^{\hat{T}},\upB^0\rrangle\notag
        \\
        &+\frac{2(C+2)\eta^2}{1-\widetilde{\calO}(C+2)\eta\tr(\upH)}\hat{T}\log(\hat{T})\llangle\widetilde{\upH}^{\hat{T}},\upB^0\rrangle\overline{\upH}^{\hat{T}}\notag
        \\
        \preceq&\left(\calI-\eta\widehat{\calG}\right)^{\hat{T}}\circ\upB_{\diag}^0+\frac{\widetilde{\calO}(C+2)\eta^2\hat{T}}{1-\widetilde{\calO}(C+2)\eta\tr(\upH)}\llangle\widetilde{\upH}^{\hat{T}},\upB^0\rrangle\overline{\upH}^{T}.
    \end{align}
    By the definition of $\widehat{\calG}$ completes the proof.
\end{proof}

Notice that in the second phase, the step size 
$\eta_t$ decays geometrically. Thus, we define the bias iterate at the end of the step-size-decaying phase as:
\begin{align}
    \widetilde{\upB}^l:=\begin{cases}
        \upB^h, & l=0,\\
        \upB^{h+Kl}, & l\in[1:L].
    \end{cases}
\end{align}
Based on the step-size iteration in Algorithm \ref{SGD} and preceding definition, we formalize the iterative process of Algorithm \ref{SGD} in Phase II as: 1) Phase $l=0$: Initialized from $\upB^0$, Algorithm \ref{SGD} executes $h$ iterations with step size $\eta_0$, yielding $\widetilde{\upB}^0$;
2) Phase $l\geq1$: Initialized from $\widetilde{\upB}^{l-1}$, Algorithm \ref{SGD} executes $K$ iterations with step size $\eta_0/2^{l}$, yielding $\widetilde{\upB}^l$. This multi-phase process terminates at $l=L$, with $\widetilde{\upB}^L = \upB^{T_2}$ as the final output.
% in state $l\geq1$, SGD is initialized from $\widetilde{\upB}^{l-1}$ and runs for $K$ steps with step-size $\eta_0/2^{l}$ and output $\widetilde{\upB}^l$; the final output is $\widetilde{\upB}^L=\upB^{T_2}$.
\begin{lemma}\label{lemma-Bias-tr-1}
    Suppose Assumption \ref{ass-d} and Assumption \ref{ass-s} hold. Under the setting of Theorem \ref{phase-II-main}, we have
    \begin{align}
        \llangle\upH,\widetilde{\upB}^l\rrangle\leq K_l:=
        \begin{cases}
            4\llangle\frac{25}{\eta_0 h}\upI_{1:N_0}+\upH_{N_0+1:M},\upB^0\rrangle, & \text{ for }\, l=0,
            \\
            4\llangle\frac{25\cdot2^l}{\eta_0 K}\upI_{1:N_0}+\upH_{N_0+1:M},\widetilde{\upB}^{l-1}\rrangle, & \text{ for }\, l\in[1:L],
        \end{cases}
    \end{align}
    for arbitrary $N_0\in[0:N]$.
\end{lemma}
\begin{proof}
    For $\llangle\upH,\widetilde{\upB}^0\rrangle$, we apply Lemma \ref{period-bias-lemma} with $\eta=\eta_0$ and $\hat{T}=h$, and use the condition that $\widetilde{\calO}(C+2)\eta\tr(\upH)\leq1/4$; For $\llangle\upH,\widetilde{\upB}^l\rrangle$ with $l\geq 2$, we apply Lemma \ref{period-bias-lemma} with $\eta=\eta_0/2^l$, $\hat{T}=K$ and $\upB^0=\widetilde{\upB}^{l-1}$, and use the condition that $\widetilde{\calO}(C+2)\eta\tr(\upH)\leq1/4$.
\end{proof}

\begin{lemma}\label{lemma-Bias-diag-2}
    Suppose Assumption \ref{ass-d} and Assumption \ref{ass-s} hold. Under the setting of Theorem \ref{phase-II-main}, we have
    \begin{align}
        \widetilde{\upB}_{\diag}^l\preceq\upR^l:=\begin{cases}
            \left(\upI-\eta_0\widehat{\upH}\right)^{h}\upB_{\diag}^0\left(\upI-\eta_0\widehat{\upH}\right)^{h}+P_0\overline{\upH}_0^h, & \text{ for }\, l=0,
            \\
            \left(\upI-\frac{\eta_0}{2^l}\widehat{\upH}\right)^{h}\widetilde{\upB}_{\diag}^{l-1}\left(\upI-\frac{\eta_0}{2^l}\widehat{\upH}\right)^{h}+P_l\overline{\upH}_l^K, & \text{ for }\, l\in[1:L],
        \end{cases}
    \end{align}
    where $\overline{\upH}_0^t:=\frac{25}{\eta_0 t}\upI_{1:N_0'}+\upH_{N_0'+1:M}$ and $\overline{\upH}_l^t:=\frac{25\cdot2^l}{\eta_0 t}\upI_{1:N_0'}+\upH_{N_0'+1:M}$ for any $t\geq1$ and arbitrary $N_0'\in[0:N]$, and $P_0:=\widetilde{\calO}(C+2)\eta_0^2h\langle\widetilde{\upH}_0^h,\upB^0\rangle$ with $\widetilde{\upH}_0^h:=\frac{25}{\eta_0 h}\upI_{1:N_0}+\upH_{N_0+1:M}$ and $P_l:=\widetilde{\calO}(C+2)(\frac{\eta_0}{2^l})^2K\langle\widetilde{\upH}_l^K,\widetilde{\upB}^{l-1}\rangle$ for $l\in[1:L]$ with $\widetilde{\upH}_l^K:=\frac{25\cdot2^l}{\eta_0 K}\upI_{1:N_0}+\upH_{N_0+1:M}$ for arbitrary $N_0\in[0:N]$
\end{lemma}
\begin{proof}
    For $\widetilde{\upB}^0$, we apply Lemma \ref{bias-diag} with $\eta=\eta_0$ and $\hat{T}=h$, and use the condition that $\widetilde{\calO}(C+2)\eta\tr(\upH)\leq1/4$. For $\widetilde{\upB}^l$ with $l\geq 2$, we apply Lemma \ref{bias-diag} with $\eta=\eta_0/2^l$, $\hat{T}=K$ and $\upB^0=\widetilde{\upB}^{l-1}$, and use the condition that $\widetilde{\calO}(C+2)\eta\tr(H)\leq1/8$.
\end{proof}
\begin{lemma}\label{phase-II-thm-p1}
    Suppose Assumption \ref{ass-d} and Assumption \ref{ass-s} hold. Under the setting of Theorem \ref{phase-II-main}, we have
    \begin{align}
        \llangle\upH,\upB^{T_2}\rrangle=\llangle\upH,\widetilde{\upB}^L\rrangle\leq e\llangle\upH,\widetilde{\upB}^1\rrangle
    \end{align}
\end{lemma}
\begin{proof}
    Consider $l\geq 1$. According to Lemma \ref{lemma-Bias-diag-2}, we obtain
    \begin{align}\label{exp-dynamic-Bias}
        \widetilde{\upB}_{\diag}^l\preceq&\left(\upI-\frac{\eta_0}{2^l}\widehat{\upH}\right)^{h}\widetilde{\upB}_{\diag}^{l-1}\left(\upI-\frac{\eta_0}{2^l}\widehat{\upH}\right)^{h}+P_l\widetilde{\upH}_l^K\notag
        \\
        \overset{\text{(a)}}{\preceq}&\widetilde{\upB}_{\diag}^{l-1}+\widetilde{\calO}(C+2)\log(K)\cdot\frac{\eta_0}{2^l}\cdot\llangle\upH,\widetilde{\upB}^{l-1}\rrangle\upI.
    \end{align}
    where (a) is derived from choosing $N_0'=N$ and $N_0=0$ in $\overline{\upH}_l^K$ and $\widetilde{\upH}_l^K$ for any $l\in[1:L]$, respectively, and $\upH_{N+1:M}\preceq\frac{\widetilde{\calO}(2^l)}{\eta_0K}\upI_{N+1:M}$. One can notice that Eq.~\eqref{exp-dynamic-Bias} implies that
    \begin{align}\label{linear-relation-bias}
        \llangle\upH,\widetilde{\upB}^l\rrangle\leq\left(1+\widetilde{\calO}(C+2)\tr(\upH)\log(K)\cdot\frac{\eta_0}{2^l}\right)\llangle\upH,\widetilde{\upB}^{l-1}\rrangle.
    \end{align}
    Therefore, we have following estimation of bias iterates using Eq.~\eqref{linear-relation-bias}:
    \begin{align}
        \llangle\upH,\widetilde{\upB}^L\rrangle\leq&\prod_{l=1}^L\left(1+\widetilde{\calO}(C+2)\tr(\upH)\log(K)\cdot\frac{\eta_0}{2^l}\right)\llangle\upH,\widetilde{\upB}^1\rrangle\notag
        \\
        \leq&\exp\left\{\widetilde{\calO}(C+2)\eta_0\tr(\upH)\log(K)\sum_{l=1}^L2^{-l}\right\}\llangle\upH,\widetilde{\upB}^1\rrangle\notag
        \\
        \leq&e\llangle\upH,\widetilde{\upB}^1\rrangle.
    \end{align}
\end{proof}
\begin{lemma}\label{phase-II-thm-p2}
    Suppose Assumption \ref{ass-d} and Assumption \ref{ass-s} hold. Under the setting of Theorem \ref{phase-II-main}, we have
    \begin{align}
        \llangle\upH,\widetilde{\upB}^{1}\rrangle\leq&8\llangle\frac{25}{\eta_0 K}\upI_{1:N_0}+\upH_{N_0+1:M},\left(\upI-\eta_0\widehat{\upH}\right)^{2h}\upB^0\rrangle\notag
        \\
        &+\widetilde{\calO}(C+2)\Gamma_K(\upH)\llangle\frac{25}{\eta_0h}\upI_{1:N_0'}+\upH_{N_0'+1:M},\upB^0\rrangle,
    \end{align}
    where $\Gamma_K(\upH):=\left(\frac{625N_0'}{K}+\frac{25\eta_0h}{K}\tr(\upH_{N_0'+1:N_0})+\eta_0^2h\tr(\upH_{N_0+1:M}^2)\right)$ for arbitrary $N\geq N_0\geq N_0'\geq 0$.
\end{lemma}
\begin{proof}
    According to Lemma \ref{lemma-Bias-tr-1}, we have
    \begin{align}
        \llangle\upH,\widetilde{\upB}^1\rrangle\leq8\llangle\frac{25}{\eta_0 K}\upI_{1:N_0}+\upH_{N_0+1:M},\widetilde{\upB}^0\rrangle,\notag
    \end{align}
    for arbitrary $N_0\in[0:N]$. Next, choosing $N_0=N_0'$ in Lemma \ref{lemma-Bias-diag-2}, we obtain
    \begin{align}
        \widetilde{\upB}_{\diag}^0\preceq&\left(\upI-\eta_0\widehat{\upH}\right)^h\upB_{\diag}^0\left(\upI-\eta_0\widehat{\upH}\right)^h\notag
        \\
        &+\widetilde{\calO}(C+2)\eta_0^2h\llangle\frac{25}{\eta_0h}\upI_{1:N_0'}+\upH_{N_0'+1:M},\upB^0\rrangle\left(\frac{25}{\eta_0h}\upI_{1:N_0'}+\upH_{N_0'+1:M}\right).\notag
    \end{align}
    Combining above two inequalities yields that
    \begin{align}
        \llangle\upH,\widetilde{\upB}^1\rrangle\leq&8\llangle\frac{25}{\eta_0 K}\upI_{1:N_0}+\upH_{N_0+1:M},\left(\upI-\eta_0\widehat{\upH}\right)^{2h}\upB^0\rrangle\notag
        \\
        &+\widetilde{\calO}(C+2)\eta_0^2h\llangle\frac{25}{\eta_0h}\upI_{1:N_0'}+\upH_{N_0'+1:M},\upB^0\rrangle\notag
        \\
        &\, \, \, \, \, \, \, \, \, \, \, \, \, \, \, \, \, \, \, \, \, \, \, \, 
        \, \, \, \, \, \, \, \, \, \, \times\llangle\frac{25}{\eta_0 K}\upI_{1:N_0}+\upH_{N_0+1:M},\frac{25}{\eta_0h}\upI_{1:N_0'}+\upH_{N_0'+1:M}\rrangle,\notag
    \end{align}
    with 
    \begin{align}
        &\llangle\frac{25}{\eta_0 K}\upI_{1:N_0}+\upH_{N_0+1:M},\frac{25}{\eta_0h}\upI_{1:N_0'}+\upH_{N_0'+1:M}\rrangle\notag
        \\
        \leq&\frac{625N_0'}{\eta_0^2hK}+\frac{25}{\eta_0K}\tr(\upH_{N_0'+1:N_0})+\tr(\upH_{N_0+1:M}^2),
    \end{align}
    when $N_0>N_0'$.
\end{proof}
\begin{theorem}\label{bias-upper-bound}
    Suppose Assumptions \ref{ass-d} and \ref{ass-s} hold. Under the setting of Theorem \ref{phase-II-main}, we have
    \begin{align}
        \llangle\upH,\upB^{T_2}\rrangle\lesssim&\llangle\frac{1}{\eta_0 K}\upI_{1:N_0}+\upH_{N_0+1:M},\left(\upI-\eta_0\widehat{\upH}\right)^{2h}\upB^0\rrangle\notag
        \\
        &+(C+2)\Gamma_K(\upH)\llangle\frac{1}{\eta_0h}\upI_{1:N_0'}+\upH_{N_0'+1:M},\upB^0\rrangle,
    \end{align}
    where $\Gamma_K(\upH):=\left(\frac{625N_0'}{K}+\frac{25\eta_0h}{K}\tr(\upH_{N_0'+1:N_0})+\eta_0^2h\tr(\upH_{N_0+1:M}^2)\right)$ for arbitrary $N\geq N_0\geq N_0'\geq 0$.
\end{theorem}
\begin{proof}
    Using Lemma \ref{phase-II-thm-p1} and Lemma \ref{phase-II-thm-p2} directly.
\end{proof}

\subsection{Proof of Convergence to Ground Truth}

\noindent\textbf{Parameter Setting}\quad We consider the parameter setting as follows:
\begin{equation}\label{para-setting-spec}
\small
    \begin{split}
&L_1=\widetilde{\calO}\left((\sigma^2+\calM^2(\upb))^2+\Hatsigmax(N)\right),\, \, \, L_2=\widetilde{\calO}(\sigma^2+\calM^2(\upb)),\, \, \, 
        D=1+\frac{L_1\Tildesigmax(N)\Barsigmin(N)}{\sigmin(N)},
    \end{split}
\end{equation}
\begin{theorem}\label{theorem-main-convergence}[General Version of Theorem \ref{theorem-3}]
	Under Assumption \ref{ass-d} and Assumption \ref{ass-s}, we consider a predictor trained by Algorithm \ref{SGD} with $T$ samples. Let $h<T$ and $T_1:=\lceil(T-h)/\log(T-h)\rceil$. Suppose there exists $N\leq M$ such that $T_1\in[\frac{L_1D}{\sigmin(N)\Barsigmin(N)}, \frac{L_2D^2}{\Tildesigmax(N)\Barsigmin^2(N)}]$ with parameter setting Eq.~\eqref{para-setting-spec} and let $\eta=\widetilde{\Theta}(\frac{\Barsigmin(N)}{\sigma^2+\calM^2(\upb)})$. Then we have
    \begin{equation}
        \begin{split}
        \calR_M(\upv^{T})-\calR_M(\upv^*)\lesssim&\frac{\sigma^2N}{T_1}+\sigma^2\eta^2(h+T_1)\sum_{i=N+1}^M\lambda_i^2(\upv_i^*)^4\notag
        \\
        &+\frac{1}{\eta T_1}\tr\left(\left(\upI_{1:N}-\frac{\eta}{4}\upH_{1:N}^*\right)^{2h}\diag\left\{(\upv_{1:N}^*)^{\odot2}\right\}\right)\notag
        \\
        &+\llangle\upH_{N+1:M}^*,\diag\left\{(\upv_{N+1:M}^*)^{\odot2}\right\}\rrangle\notag
        \\
        &+\left(\frac{N}{T_1}+\eta^2h\tr\left((\upH_{N+1:M}^*)^2\right)\right)\llangle\frac{1}{\eta h}\upI_{1:N}+\upH_{N+1:M}^*,\diag\left\{(\upv^*)^{\odot2}\right\}\rrangle,\notag
        \end{split}
    \end{equation}
    with probability at least 0.95. Otherwise, let $T_1\in[\frac{L_1D}{\sigmin(M)\Barsigmin(M)},+\infty)$ with parameter setting Eq.~\eqref{para-setting-spec} and $\eta=\widetilde{\Theta}(\frac{\Barsigmin(M)}{\sigma^2+\calM^2(\upb)})$. Then we have
    \begin{equation}
        \begin{split}
        \calR_M(\upv^{T})-\calR_M(\upv^*)\lesssim&\frac{\sigma^2M}{T_1}+\frac{1}{\eta T_1}\tr\left(\left(\upI-\frac{\eta}{4}\upH^*\right)^{2h}\diag\left\{(\upv_{1:M}^*)^{\odot2}\right\}\right)\notag
        \\
        &+\frac{M}{\eta hT_1}\tr\left(\diag\left\{(\upv_{1:M}^*)^{\odot2}\right\}\right),\notag
        \end{split}
    \end{equation}
    with probability at least 0.95.
\end{theorem}
\begin{proof}
    Combining Theorem \ref{theorem_1} and Theorem \ref{phase-II-main}, we complete the proof.
\end{proof}

\subsection{Proof of Lower Bound}
As established in Phase I, $\upv^{T_1}$ satisfies the inequality $\overline{\upb} \leq \upv^{T_1} \leq \widehat{\upb}$ with high probability. Here, $\widehat{\upb}$ is defined as $\widehat{\upb}^{\top}=(\frac{3}{2}(\upv_{1:N}^*)^{\top},3(\upv_{N+1:M}^*)^{\top})$, while $\overline{\upb}$ is given by $\overline{\upb}^{\top}=(\frac{1}{2}(\upv_{1:N}^*)^{\top},\mathbf{0}^{\top})$. We proceed by introducing the required preliminary concepts. A Markov chain $\{\breve{\upv}^t\}_{t=0}^{T_2}$ is constructed with initialization $\breve{\upv}^0$ satisfying $\overline{\upb} \leq \breve{\upv}^0 \leq \widehat{\upb}$. The update rule is defined by
\begin{align}\label{eq-bv}
     \breve{\upv}^{t+1}=\breve{\upv}^t-\eta_t\upH_{\breve{\upv}}^t\left(\breve{\upv}^t-\upv_{1:M}^*\right)+\eta_t\upR_{\breve{\upv}}^t\Pi_M\upx^t, \quad \forall t\in[0:T_2-1],\notag
\end{align}
% if $\overline{\upb}\leq\breve{\upv}^t\leq\widehat{\upb}$, let
% \begin{align}
%     \breve{\upv}^{t+1}=\breve{\upv}^t-\eta_t\upH_{\breve{\upv}}^t\left(\breve{\upv}^t-\upv_{1:M}^*\right)+\eta_t\upR_{\breve{\upv}}^t\Pi_M\upx^t,\notag
% \end{align}
% otherwise, let 
% \begin{align}
%     \breve{\upv}^{\tau+1}=\breve{\upv}^{\tau}-\eta_{\tau}\breve{\upH}^{\tau}(\breve{\upv}^{\tau}-\upv_{1:M}^*)+\eta_{\tau}\breve{\upR}^{\tau}\Pi_M\upx^{\tau},\quad\forall \tau\in[t:T_2-1],\notag
% \end{align}
where $\upH_{\breve{\upv}}^{t}$ and $\upR_{\breve{\upv}}^t$ satisfy: 
\begin{enumerate}
    \item If $\overline{\upb}\leq\breve{\upv}^t\leq\widehat{\upb}$, $\upH_{\breve{\upv}}^{t}=(\breve{\upv}^t\odot\Pi_M\upx^t)\otimes((\breve{\upv}^t+\upv_{1:M}^*)\odot\Pi_M\upx^t)$ and $\upR_{\breve{\upv}}^t=(\xi^t+\sum_{i=M+1}^{\infty}\upx_i^t(\upv_i^*)^2)\diag\{\breve{\upv}^t\}$,
    \item Otherwise, for any $\tau\in[t:T_2-1]$,  $\upH_{\breve{\upv}}^{\tau}=\frac{25}{4}(\upv_{1:M}^*\odot\Pi_{M}\upx^{\tau})\otimes(\upv_{1:M}^*\odot\Pi_{M}\upx^{\tau})$ and $\upR_{\breve{\upv}}^{\tau}=(\xi^{\tau}+\sum_{i=M+1}^{\infty}\upx_i^{\tau}(\upv_i^*)^2)$ $\diag\{\overline{\upb}\}$.
\end{enumerate}
Let $\breve{\upw}^t:=\breve{\upv}^t-\upv_{1:M}^*$ be the error vector, and let $t_s:=\inf\{t\mid \breve{\upv}^t\nleqslant\widehat{\upb}\bigvee\breve{\upv}^t\ngeqslant\overline{\upb}\}$ be the stopping time. According to Eq.~\eqref{eq-bv}, $\{\breve{\upw}^t\}_{t=1}^{T_2}$ is recursively defined by
\begin{align}
		\breve{\upw}^{t+1}=\left(\upI-\eta_t\upH_{\breve{\upv}}^t\right)\breve{\upw}^t+\eta_t\upR_{\breve{\upv}}^t\Pi_M\upx^t, \notag
\end{align}
% Analogous to Phase II analysis, the dynamics of $\breve{\upw}^t$ can be decomposed into two random processes,
% \begin{align}
%     \breve{\upw}^t=\breve{\upw}_{\bi}^t+\breve{\upw}_{\var}^t,
% \end{align}
% for any $t\in[0:T_2]$, where $\{\breve{\upw}_{\var}^t\}_{t=1}^{T_2}$ is recursively defined by
% \begin{align}
% 		\breve{\upw}_{\var}^{t+1}=\left(\upI-\eta_t\upH_{\breve{\upv}}^t\right)\breve{\upw}_{\var}^t+\eta_t\upR_{\breve{\upv}}^t\Pi_M\upx^t, \notag
% \end{align}
% for any $t\in[0:T_2-1]$ with $\breve{\upw}_{\var}^0=0$ and $\{\breve{\upw}_{\bi}^t\}_{t=1}^{T_2}$ is recursively defined by
% \begin{align}
% 		\breve{\upw}_{\bi}^{t+1}=\left(\upI-\eta_t\upH_{\breve{\upv}}^t\right)\breve{\upw}_{\bi}^t, \notag
% \end{align}
% for any $t\in[0:T_2-1]$ with  $\breve{\upw}_{\bi}^0=\breve{\upv}^0-\upv_{1:M}^*$. 
We define $\breve{\upV}^t=\bbE\left[\breve{\upw}^t\otimes\breve{\upw}^t\right]$. By referring to the definitions of $\calH_{\cdot}^t$, $\widetilde{\calH}_{\cdot}^t$, $\calG_{\cdot}^t$, and $\widetilde{\calG}_{\cdot}^t$ established in Phase II, we derive the iterative relationship governing the sequence $\{\breve{\upV}^t\}_{t=0}^{T_2}$:
\begin{align}
	% \begin{cases}
 %        \breve{\upB}^{t+1}&=\left(\calI-\eta_t\calG_{\breve{\upv}}^t\right)\circ\breve{\upB}^t,
	% 	\\
		\breve{\upV}^{t+1}&=\bbE\left[\left(\calI-\eta_t\calG_{\breve{\upv}}^t\right)\circ\left(\breve{\upw}^t\otimes\breve{\upw}^t\right)\right]+\eta_t^2\upSigma_{\breve{\upv}}^t,
	% \end{cases}
\end{align}
for $t\in[0:T_2-1]$ with $\upV^0=\left(\upw^0-\upv_{1:M}^*\right)\otimes\left(\upw^0-\upv_{1:M}^*\right)$. If $t<t_s$, $\upSigma_{\breve{\upv}}^t=\sigma^2\upLambda\diag\{\breve{\upv}^{t\odot2}\}$; otherwise, $\upSigma_{\breve{\upv}}^{\tau}=\sigma^2\upLambda\diag\{\overline{\upb}^{\odot2}\}$ for any $\tau\geq t$. According to the definitions above, we obtain following estimation of last-iterate function value:
\begin{align}\label{lower-bound-I}
    \bbE\left[\calR_M(\breve{\upw}^{T_2})-\calR_M(\upv_{1:M}^*)\right]\geq\frac{1}{24}\llangle\breve{\upH},\bbE\left[\breve{\upw}^{T_2}\otimes\breve{\upw}^{T_2}\right]\rrangle\geq\frac{1}{24}\llangle\breve{\upH},\breve{\upV}^{T_2}\rrangle,
\end{align}
where $\breve{\upH}:=12\upLambda\diag\{\upv_{1:M}^*\odot\upv_{1:M}^*\}$. We define $\breve{\calG}^i:=\breve{\upH}\otimes\upI+\upI\otimes\breve{\upH}-\eta_i\breve{\upH}\otimes\breve{\upH}$. In order to derive the variance lower bound, we have the following estimation:
\begin{theorem}[General Version of Theorem \ref{lower-bound}]
    Under Assumptions \ref{ass-d} and \ref{ass-s}, we consider a predictor trained by Algorithm \ref{SGD} with iteration number $T$. Suppose there exists $N\leq M$ such that $T_1\in[\widetilde{\calO}(\frac{\sigma^2+\mathcal{M}^2(\upb)}{\eta\sigmin(N)}),\widetilde{\Theta}(\frac{\Tildesigmax^{-1}(N)}{\eta^2(\sigma^2+\mathcal{M}^2(\upb))})]$, where $\eta\leq\widetilde{\Theta}(\frac{\Barsigmin(N)}{(\sigma^2+\mathcal{M}^2(\upb))^2})$ and $T_1:=\lceil(T-h)/\log(T-h)\rceil$ with $h\geq T_1$. Then we have
    \begin{align}
    \bbE\left[\calR_M(\upv^{T})-\calR_M(\upv_{1:M}^*)\right]\gtrsim\sigma^2\left(\frac{H_1}{T_1}+\eta\sum_{i=H_1+1}^{H_2}\lambda_i(\upv_i^*)^2+\eta^2h\sum_{i=H_2+1}^{N}\lambda_i^2(\upv_i^*)^4\right),\notag
\end{align}
where $H_1:=\min\{N,\max\{i\mid\lambda_i(\upv_i^*)^2\geq\frac{1}{12\eta T_1}\}\}$ and $H_2:=\min\{N,\max\{i\mid\lambda_i(\upv_i^*)^2\geq\frac{1}{12\eta h}\}\}$. Otherwise, let $T_1\in[\widetilde{\calO}(\frac{\sigma^2+\mathcal{M}^2(\upb)}{\eta\sigmin(M)}),+\infty)$, where $\eta\leq\widetilde{\Theta}(\frac{\Barsigmin(M)}{(\sigma^2+\mathcal{M}^2(\upb))^2})$ and $T_1:=\lceil(T-h)/\log(T-h)\rceil$ with $h\geq T_1$. Then we have
    \begin{align}
    \bbE\left[\calR_M(\upv^{T})-\calR_M(\upv_{1:M}^*)\right]\gtrsim\sigma^2\left(\frac{H_1'}{T_1}+\eta\sum_{i=H_1'+1}^{H_2'}\lambda_i(\upv_i^*)^2+\eta^2h\sum_{i=H_2'+1}^{N}\lambda_i^2(\upv_i^*)^4\right),\notag
\end{align}
where $H_1':=\min\{M,\max\{i\mid\lambda_i(\upv_i^*)^2\geq\frac{1}{12\eta T_1}\}\}$ and $H_2':=\min\{M,\max\{i\mid\lambda_i(\upv_i^*)^2\geq\frac{1}{12\eta h}\}\}$.
\end{theorem}
\begin{proof}
    Setting $\eta_0 = \eta$ yields 
    \begin{align}
        \breve{\upV}_{\diag}^{t+1}=&\left(\bbE\left[\left(\calI-\eta_t\widetilde{\calG}_{\breve{\upv}}^t\right)\circ\left(\breve{\upw}^t\otimes\breve{\upw}^t\right)\right]\right)_{\diag}+\eta_t^2\left(\bbE\left[\left(\calH_{\breve{\upv}}^t-\widetilde{\calH}_{\breve{\upv}}^t\right)\circ\left(\breve{\upw}^t\otimes\breve{\upw}^t\right)\right]\right)_{\diag}+\eta_t^2\Sigma_{\breve{\upv}}^t\notag
        \\
        \succeq&\left(\calI-\eta_t\breve{\calG}^t\right)\circ\breve{\upV}_{\diag}^t+\eta_t^2\sigma^2\upLambda\diag\left\{\overline{\upb}^{\odot2}\right\}.\notag
    \end{align}
    According to the recursive step above, we obtain
    \begin{align}\label{lower-bound-proof-I}
        \breve{\upV}^{T_2}
        % \succeq&\sigma^2\sum_{t=1}^{T_2}\eta_t^2\prod_{i=t+1}^{T_2}\left(\calI-\eta_i\widetilde{\calG}_{\breve{\upv}}^i\right)\circ\upLambda\diag\left\{\overline{\upb}^{\odot2}\right\}\notag
        % \\
        \succeq&\sigma^2\sum_{t=1}^{T_2}\eta_t^2\prod_{i=t+1}^{T_2}\left(\upI-\eta_i\breve{\upH}\right)^2\upLambda\diag\left\{\overline{\upb}^{\odot2}\right\}\notag
        \\
        \succeq&\sigma^2\underbrace{\sum_{t=1}^{T_2}\eta_t^2\prod_{i=t+1}^{T_2}\left(\upI-2\eta_i\breve{\upH}\right)\upLambda\diag\left\{\overline{\upb}^{\odot2}\right\}}_{\calcolI}.
    \end{align}
    Recalling the step size decay rule in Algorithm \ref{SGD}, we have
    \begin{align}\label{lower-bound-proof-2}
        \calcolI=&\eta_0^2\sum_{i=1}^h\left(\upI-2\eta_0\breve{\upH}\right)^{h-i}\prod_{j=1}^{L-1}\left(\upI-\frac{\eta_0}{2^{j-1}}\breve{\upH}\right)^K\upLambda\diag\left\{\overline{\upb}^{\odot2}\right\}\notag
	\\
	&+\sum_{l=1}^{L-1}\left(\frac{\eta_0}{2^l}\right)^2\sum_{i=1}^K\left(\upI-\frac{\eta_0}{2^{l-1}}\breve{\upH}\right)^{K-i}\prod_{j=l+1}^{L-1}\left(\upI-\frac{\eta_0}{2^{j-1}}\breve{\upH}\right)^K\upLambda\diag\left\{\overline{\upb}^{\odot2}\right\}\notag
	\\
	=&\frac{\eta_0^2}{12}\sum_{i=1}^h\left(\upI_{1:N}-2\eta_0\breve{\upH}_{1:N}\right)^{h-i}\prod_{j=1}^{L-1}\left(\upI_{1:N}-\frac{\eta_0}{2^{j-1}}\breve{\upH}_{1:N}\right)^K\breve{\upH}_{1:N}\notag
	\\
	&+\frac{1}{12}\sum_{l=1}^{L-1}\left(\frac{\eta_0}{2^l}\right)^2\sum_{i=1}^K\left(\upI_{1:N}-\frac{\eta_0}{2^{l-1}}\breve{\upH}_{1:N}\right)^{K-i}\prod_{j=l+1}^{L-1}\left(\upI_{1:N}-\frac{\eta_0}{2^{j-1}}\breve{\upH}_{1:N}\right)^K\breve{\upH}_{1:N}\notag
	\\
	=&\frac{\eta_0}{24}\left(\upI_{1:N}-\left(\upI_{1:N}-2\eta_0\breve{\upH}_{1:N}\right)^h\right)\left(\prod_{j=1}^{L-1}\left(\upI_{1:N}-\frac{\eta_0}{2^{j-1}}\breve{\upH}_{1:N}\right)\right)^K\notag
	\\
	&+\sum_{l=1}^{L-1}\frac{\eta_0}{12\cdot 2^{l+1}}\left(\upI_{1:N}-\left(\upI_{1:N}-\frac{\eta_0}{2^{l-1}}\breve{\upH}_{1:N}\right)^K\right)\left(\prod_{j=l+1}^{L-1}\left(\upI_{1:N}-\frac{\eta_0}{2^{j-1}}\breve{\upH}_{1:N}\right)\right)^K\notag
	\\
	\overset{\text{(a)}}{\geq}&\frac{\eta_0}{24}\left(\upI_{1:N}-\left(\upI_{1:N}-2\eta_0\breve{\upH}_{1:N}\right)^h\right)\left(\upI_{1:N}-2\eta_0\breve{\upH}_{1:N}\right)^K\notag
	\\
	&+\sum_{l=1}^{L-1}\frac{\eta_0}{12\cdot 2^{l+1}}\left(\upI_{1:N}-\left(\upI_{1:N}-\frac{\eta_0}{2^{l-1}}\breve{\upH}_{1:N}\right)^K\right)\left(\upI_{1:N}-\frac{\eta_0}{2^{l-1}}\breve{\upH}_{1:N}\right)^K,
    \end{align}
    where (a) is derived from following inequality
\begin{align}
	\prod_{i=l+1}^{L-1}\left(\upI_{1:N}-\frac{\eta_0}{2^{i-1}}\breve{\upH}_{1:N}\right)\geq\upI_{1:N}-\sum_{i=l+1}^{L-1}\frac{\eta_0}{2^{i-1}}\breve{\upH}\geq\upI_{1:N}-\frac{\eta_0}{2^{l-1}}\breve{\upH}_{1:N}.\notag
\end{align}
When $h > K$, an auxiliary function analogous to [Lemma D.1, \citet{wu2022last}]can be applied:
\begin{align}
    f(x):=\frac{x}{2}\left(1-\left(1-2x\right)^h\right)(1-2x)^K+\sum_{l=1}^{L-1}\frac{x}{2^{l+1}}\left(1-\left(1-\frac{x}{2^{l-1}}\right)^K\right)\left(1-\frac{x}{2^{l-1}}\right)^K.\notag
\end{align}
Then, we obtain
\begin{align}\label{lower-bound-proof-III}
    f(\eta_0\breve{\upH})\succeq\frac{1}{4800K}\upI_{1:H_1}+\frac{\eta_0}{480}\breve{\upH}_{H_1+1:H_2}+\frac{\eta_0^2h}{480}\breve{\upH}_{H_2+1:N}^2,
\end{align}
where $H_1:=\min\{N,\max\{i\mid\lambda_i(\upv_i^*)^2\geq\frac{1}{12\eta_0K}\}\}$ and $H_2:=\min\{N,\max\{i\mid\lambda_i(\upv_i^*)^2\geq\frac{1}{12\eta_0h}\}\}$. Therefore, using Eq.~\eqref{lower-bound-I}-Eq.~\eqref{lower-bound-proof-III}, we derive 
\begin{align}
    \bbE\left[\calR_M(\breve{\upv}^{T_2})-\calR_M(\upv_{1:M}^*)\right]\geq&\frac{\sigma^2}{11520}\llangle\breve{\upH},\frac{1}{10K}\breve{\upH}_{1:H_1}^{-1}+\eta_0\upI_{H_1+1:H_2}+\eta_0^2h\breve{\upH}_{H_2+1:N}\rrangle\notag
    \\
    =&\frac{\sigma^2}{11520}\left(\frac{H_1}{10K}+12\eta_0\sum_{i=H_1+1}^{H_2}\lambda_i(\upv_i^*)^2+144\eta_0^2h\sum_{i=H_2+1}^{N}\lambda_i^2(\upv_i^*)^4\right).\notag
\end{align}
According to Lemma \ref{high-probability-phase-II}, we have $\mathbb{P}(t_s\leq T_2)\leq\delta$, which implies that 
\begin{align}\label{lower-bound-proof-IV}
    &\bbE\left[\calR_M(\breve{\upv}^{T_2})-\calR_M(\upv_{1:M}^*)\mid t_s>T_2\right]\notag
    \\
    \geq&\bbE\left[\calR_M(\breve{\upv}^{T_2})-\calR_M(\upv_{1:M}^*)\right]-\sum_{i=1}^{T_2}\bbP(t_s=i)\bbE\left[\calR_M(\breve{\upw}^{T_2})-\calR_M(\upv_{1:M}^*)\mid t_s=i\right]\notag
    \\
    \overset{\text{(b)}}{\geq}&\frac{\sigma^2}{23040}\left(\frac{H_1}{10K}+12\eta_0\sum_{i=H_1+1}^{H_2}\lambda_i(\upv_i^*)^2+144\eta_0^2h\sum_{i=H_2+1}^{N}\lambda_i^2(\upv_i^*)^4\right).
\end{align}
Since $\delta$ is sufficiently small, (b) is drawn from two key observations: 1) $\breve{\upv}^{t_s}$ resides in a bounded neighborhood of $\widehat{\upb}$ or $\overline{\upb}$; 2) the risk upper bound for SGD established in [Theorem 4.1, \citet{wu2022last}]. The lower bound established in Eq.~\eqref{lower-bound-proof-IV} is uniformly valid for all $\breve{\upv}^0\in[\overline{\upb},\widehat{\upb}]$, as it remains independent of the initial condition $\breve{\upv}^0$. In particular, for $t_s > T_2$, the trajectory $\{\breve{\upv}^t\}_{t=0}^{T_2}$ coincides with Algorithm \ref{SGD}'s iterations over $[T_1, T]$, given the initialization $\breve{\upv}^0 = \upv^{T_1} \in [\overline{\upb}, \widehat{\upb}]$. Then, we have
\begin{align}\label{lower-bound-proof-V}
    &\min_{\overline{\upb}\leq\upv^{T_1}\leq\widehat{\upb}}\bbE\left[\calR_M(\upv^{T})-\calR_M(\upv_{1:M}^*)\mid \upv^{T_1}\right]\notag
    \\
    \geq&(1-\delta)\min_{\overline{\upb}\leq\upv^{T_1}\leq\widehat{\upb}}\bbE\left[\calR_M(\breve{\upv}^{T_2})-\calR_M(\upv_{1:M}^*)\mid t_s>T_2,\breve{\upv}^0 = \upv^{T_1}\right]\notag
    \\
    \gtrsim&\sigma^2\left(\frac{H_1}{K}+\eta_0\sum_{i=H_1+1}^{H_2}\lambda_i(\upv_i^*)^2+\eta_0^2h\sum_{i=H_2+1}^{N}\lambda_i^2(\upv_i^*)^4\right).
    % \notag
    % \\
    % \geq&\frac{\sigma^2}{46080}\left(\frac{T_1}{10K}+12\eta_0\sum_{i=T_1+1}^{T_2}\lambda_i(\upv_i^*)^2+144\eta_0^2h\sum_{i=T_2+1}^{N}\lambda_i^2(\upv_i^*)^4\right).
\end{align}
Noticing that $\upv^{T_1}\in[\overline{\upb}:\widehat{\upb}]$ occurs with probability at least $1-\delta$, and combining Eq.~\eqref{lower-bound-proof-IV} with Eq.~\eqref{lower-bound-proof-V}, we obtain
\begin{align}
    \bbE\left[\calR_M(\upv^{T})-\calR_M(\upv_{1:M}^*)\right]\geq&(1-\delta)\min_{\overline{\upb}\leq\upv^{T_1}\leq\widehat{\upb}}\bbE\left[\calR_M(\upv^{T})-\calR_M(\upv_{1:M}^*)\mid\upv^{T_1}\right]\notag
    \\
    \gtrsim&\sigma^2\left(\frac{H_1}{K}+\eta_0\sum_{i=H_1+1}^{H_2}\lambda_i(\upv_i^*)^2+\eta_0^2h\sum_{i=H_2+1}^{N}\lambda_i^2(\upv_i^*)^4\right),\notag
\end{align}
where $H_1:=\min\{N,\max\{i\mid\lambda_i(\upv_i^*)^2\geq\frac{1}{12\eta_0K}\}\}$ and $H_2:=\min\{N,\max\{i\mid\lambda_i(\upv_i^*)^2\geq\frac{1}{12\eta_0h}\}\}$.
\end{proof}
